# Supplementary material for: Algorithms of very high space-time orders of accuracy for hyperbolic equations in the semidiscrete WENO-DeC framework
Source: arXiv:2501.12994 source file (2025-05-07)
Supplement: Supplementary file 1 [file supplementary_material.tex]

\documentclass[english]{article} 
\usepackage[absolute,overlay]{textpos} 
\usepackage{amsthm}
\usepackage{amsmath}
\usepackage{amssymb}
\usepackage[utf8]{inputenc}
\usepackage[english]{babel}
\usepackage{graphicx}
\usepackage{geometry}
\usepackage{caption}
\usepackage{subcaption}
\usepackage{pdfpages}
\usepackage{comment}
\usepackage{bm}
\usepackage{etoolbox}
\usepackage{mathtools}
\usepackage{tikz}

\usepackage{algpseudocode}
\usepackage{algorithm}
\usepackage{mathrsfs} 
\usepackage{multirow}

\usepackage{pgfplots}
\usepackage{pgfplotstable}
\usepackage{stmaryrd} 

\usepackage{hyperref}

\usepackage{booktabs}

%%%%%%%%%%%%%%%%%%%%
%BIBLIOGRAPHY
%%%%%%%%%%%%%%%%%%%%
%\usepackage[numbers]{natbib}  % For numeric citations; omit [numbers] for author-year
\usepackage[style=numeric, giveninits=true, sorting=none, maxnames=99]{biblatex}
\addbibresource{sn-bibliography.bib}  % Your .bib file

\usepackage[noabbrev,capitalise]{cleveref}
\crefformat{appendix}{#2#1#3}

\usetikzlibrary{fillbetween}
\usepgfplotslibrary{fillbetween}

\usetikzlibrary{shapes.misc}
\usetikzlibrary{math} 

\usetikzlibrary{arrows}

\definecolor{darkspringgreen}{rgb}{0., 0.55, 0.3}
\definecolor{dartmouthgreen}{rgb}{0.05, 0.5, 0.06}
\definecolor{etonblue}{rgb}{0.59, 0.78, 0.64}
\definecolor{airforceblue}{rgb}{0., 0.4, 0.66}
\definecolor{arylideyellow}{rgb}{0.91, 0.84, 0.42}
\definecolor{emerald}{rgb}{0.31, 0.78, 0.47}
\definecolor{uclagold}{rgb}{1.0, 0.7, 0.0}
\definecolor{cadmiumorange}{rgb}{0.93, 0.53, 0.18}

%\newtheorem{theorem}{Theorem}
%\numberwithin{theorem}{section}
%\newtheorem{definition}{Definition}
%\numberwithin{definition}{section}
%\newtheorem{remark}{Remark}
%\numberwithin{remark}{section}
%\newtheorem{proposition}[theorem]{Proposition}
%\newtheorem{lemma}[theorem]{Lemma}
%\newtheorem{corollary}[theorem]{Corollary}

\theoremstyle{thmstyleone}

\theoremstyle{thmstyletwo}

\theoremstyle{thmstylethree}

\newcommand{\uvec}[2][3]{\boldsymbol{#2\mkern-#1mu}\mkern#1mu}

%\newcommand{\spacestuff}[0]{\boldsymbol{\phi}_i}

 %phi space _i
 %phi space _i
 %psi time ^m
 %psi time ^m
%THE FOLLOWING IS  ^l TO AVOID CONFUSION WITH u_n
 %theta space time 

%ADER-FV
 %predictor
 %corrector 

%Temperature
%\newcommand{\Temp}{\tau}

  %PNPM schemes

%\DeclarePairedDelimiter\abs{\lvert}{\rvert}

\begin{document}
\author{L. Micalizzi\footnote{Affiliation: Department of Mathematics, North Carolina State University, SAS Hall, 2108, 2311 Stinson Dr, Raleigh, NC 27607, United States. Email: lmicali@ncsu.edu}, and E. F. Toro\footnote{Affiliation: Laboratory of Applied Mathematics, DICAM, University of Trento, Via Mesiano 77, 38123 Trento, Italy. Email: eleuterio.toro@unitn.it}}
\title{Algorithms of very high space--time orders of accuracy for hyperbolic equations in the semidiscrete WENO--DeC framework\\ Supplementary Material}

\maketitle

\section*{Introduction}
In this supplementary material, we report results, which were omitted in the main manuscript to prevent excessive length.
The omitted results concern simulations on the one--dimensional Euler equations.
In Section~\ref{sec:Euler_1d_sin4}, we report the convergence tables for the density obtained with all settings resulting from coupling reconstruction of conserved (``cons.'' in the labels) or characteristic variables (``char.'' in the labels) and Rusanov (``Rus'' in the labels) or exact Riemann solver (``Ex.RS'' in the labels) numerical flux.
In Sections~\ref{sec:Euler_1d_RP1},~\ref{sec:Euler_1d_RP2},~\ref{sec:Euler_1d_RP3},~\ref{sec:Euler_1d_RP4} and~\ref{sec:Euler_1d_RP5}, we report the results on the density obtained through all settings on the Riemann problems, taken from~\cite{ToroBook}, considered in the main manuscript.
Finally, in Section~\ref{sec:Euler_1d_titarev_toro}, we report the results on the density obtained through all settings on the modified shock--turbulence interaction problem considered in the main manuscript.

For convenience, we recall here the relevant informations related to the tests. In fact, the ones concerning the Riemann problems are reported in Table~\ref{tab:Euler_1d_RP}, where $x_d$ represents the location of the discontinuity at the beginning of the simulation. For all such Riemann problems, the spatial domain is $\Omega:=[0,1]$, transmissive boundary conditions are considered. 
Missing lines in the plots reported for such tests are associated with simulation crashes for the related configurations.

\begin{table}
	\centering
	\begin{tabular}{|c||c|c|c||c|c|c||c||c|}
		\hline
		Test& $\rho_L$ & $u_L$ & $p_L$& $\rho_R$& $u_R$ & $p_R$ & $x_d$ & $T_f$\\\hline\hline
		1   &      1.0 &  0.75 &   1.0&    0.125&   0.0 &  0.1  &  0.3  & 0.2 \\
		\hline
		2   &      1.0 &  -2.0 &   0.4&      1.0&   2.0 &  0.4  &  0.5 & 0.15 \\
		\hline
		Relaxed 2  &      1.0 &  -1.0 &   0.4&      1.0&   1.0 &  0.4  & 0.5  &  0.15 \\
		\hline
		3   &      1.0 &   0.0 &1000.0&      1.0&   0.0 & 0.01  & 0.5  & 0.012 \\
		\hline
		4   &  5.99924 &19.5975&460.894& 5.99242&-6.19633&46.0950 & 0.4  & 0.035 \\
		\hline
		5   &     1.0  &-19.59745&1000.0& 1.0 & -19.59745 & 0.01 &  0.8 &  0.012\\
		\hline
	\end{tabular}
	\caption{Test informations for Riemann problems 1, 2 (and relaxed 2), 3, 4, 5. A relaxed version of Riemann problem 2 has been investigated in this work}\label{tab:Euler_1d_RP}
\end{table}

\section{Advection of smooth density}\label{sec:Euler_1d_sin4}
This test, presented in~\cite{toro2005tvd}, is characterized by the following initial condition
\begin{align}
	\begin{cases}
		\rho_0(x)&:=2+\sin^4{\left(\pi x\right)},\\
		u_0(x)&:=u_\infty, \\
		p_0(x)&:=p_\infty,
	\end{cases}
\end{align}
with $u_\infty:=1$ and $p_\infty:=1.$
The spatial domain is $\Omega:=[-1,1]$, and periodic boundary conditions are considered.
The exact solution is $\uvec{u}(x,t):=\uvec{u}_0(x-u_{\infty}t)$.
In the convergence analysis, $C_{CFL}:=0.95$ and $T_f:=2$ have been considered. 

In Tables~\ref{tab:Euler_1d_convergence_tables_WENO_DeC_cons_rusanov},~\ref{tab:Euler_1d_convergence_tables_WENO_SSPRK3_cons_rusanov},~\ref{tab:Euler_1d_convergence_tables_WENO_SSPRK4_cons_rusanov},~\ref{tab:Euler_1d_convergence_tables_WENO_mSSPRK3_cons_rusanov}, and~\ref{tab:Euler_1d_convergence_tables_WENO_mSSPRK4_cons_rusanov}, we report the convergence tables for reconstruction of conserved variables and Rusanov with WENO--DeC, WENO--SSPRK3, WENO--SSPRK4, WENO--mSSPRK3, and WENO--mSSPRK4 respectively.
In Tables~\ref{tab:Euler_1d_convergence_tables_WENO_DeC_cons_exact},~\ref{tab:Euler_1d_convergence_tables_WENO_SSPRK3_cons_exact},~\ref{tab:Euler_1d_convergence_tables_WENO_SSPRK4_cons_exact},~\ref{tab:Euler_1d_convergence_tables_WENO_mSSPRK3_cons_exact}, and~\ref{tab:Euler_1d_convergence_tables_WENO_mSSPRK4_cons_exact}, we report the convergence tables for reconstruction of conserved variables and exact Riemann solver with WENO--DeC, WENO--SSPRK3, WENO--SSPRK4, WENO--mSSPRK3, and WENO--mSSPRK4 respectively.
In Tables~\ref{tab:Euler_1d_convergence_tables_WENO_DeC_char_rusanov},~\ref{tab:Euler_1d_convergence_tables_WENO_SSPRK3_char_rusanov},~\ref{tab:Euler_1d_convergence_tables_WENO_SSPRK4_char_rusanov},~\ref{tab:Euler_1d_convergence_tables_WENO_mSSPRK3_char_rusanov}, and~\ref{tab:Euler_1d_convergence_tables_WENO_mSSPRK4_char_rusanov}, we report the convergence tables for reconstruction of characteristic variables and Rusanov with WENO--DeC, WENO--SSPRK3, WENO--SSPRK4, WENO--mSSPRK3, and WENO--mSSPRK4 respectively.
In Tables~\ref{tab:Euler_1d_convergence_tables_WENO_DeC_char_exact},~\ref{tab:Euler_1d_convergence_tables_WENO_SSPRK3_char_exact},~\ref{tab:Euler_1d_convergence_tables_WENO_SSPRK4_char_exact},~\ref{tab:Euler_1d_convergence_tables_WENO_mSSPRK3_char_exact}, and~\ref{tab:Euler_1d_convergence_tables_WENO_mSSPRK4_char_exact}, we report the convergence tables for reconstruction of characteristic variables and exact Riemann solver with WENO--DeC, WENO--SSPRK3, WENO--SSPRK4, WENO--mSSPRK3, and WENO--mSSPRK4 respectively.

Let us notice that Table~\ref{tab:Euler_1d_convergence_tables_WENO_DeC_char_exact} is reported in the main document; we report it also here for the sake of completeness.

\begin{table}[htbp]
	\centering
	\caption{Euler equations, Advection of smooth density: convergence tables for WENO--DeC with reconstruction of conserved variables and Rusanov}
	\label{tab:Euler_1d_convergence_tables_WENO_DeC_cons_rusanov}
	\scalebox{0.65}{ % Adjust the scaling factor as needed
		% [inline block 0: 20 envs, 93169 chars -> data_tex | \begin{tabular}{c c c c c c c c} 			\toprule...]
}
\end{table}

\section{Riemann problem 1 (Modified Sod)}\label{sec:Euler_1d_RP1}
In Figure~\ref{fig:Euler_1d_RP1_zoom_density}, we report the results obtained for the density for all settings on Riemann problem 1 with $C_{CFL}:=0.95$.

\begin{figure}[htbp]
	\centering
	\begin{subfigure}[b]{0.8\textwidth}
		\centering
		\includegraphics[width=\textwidth]{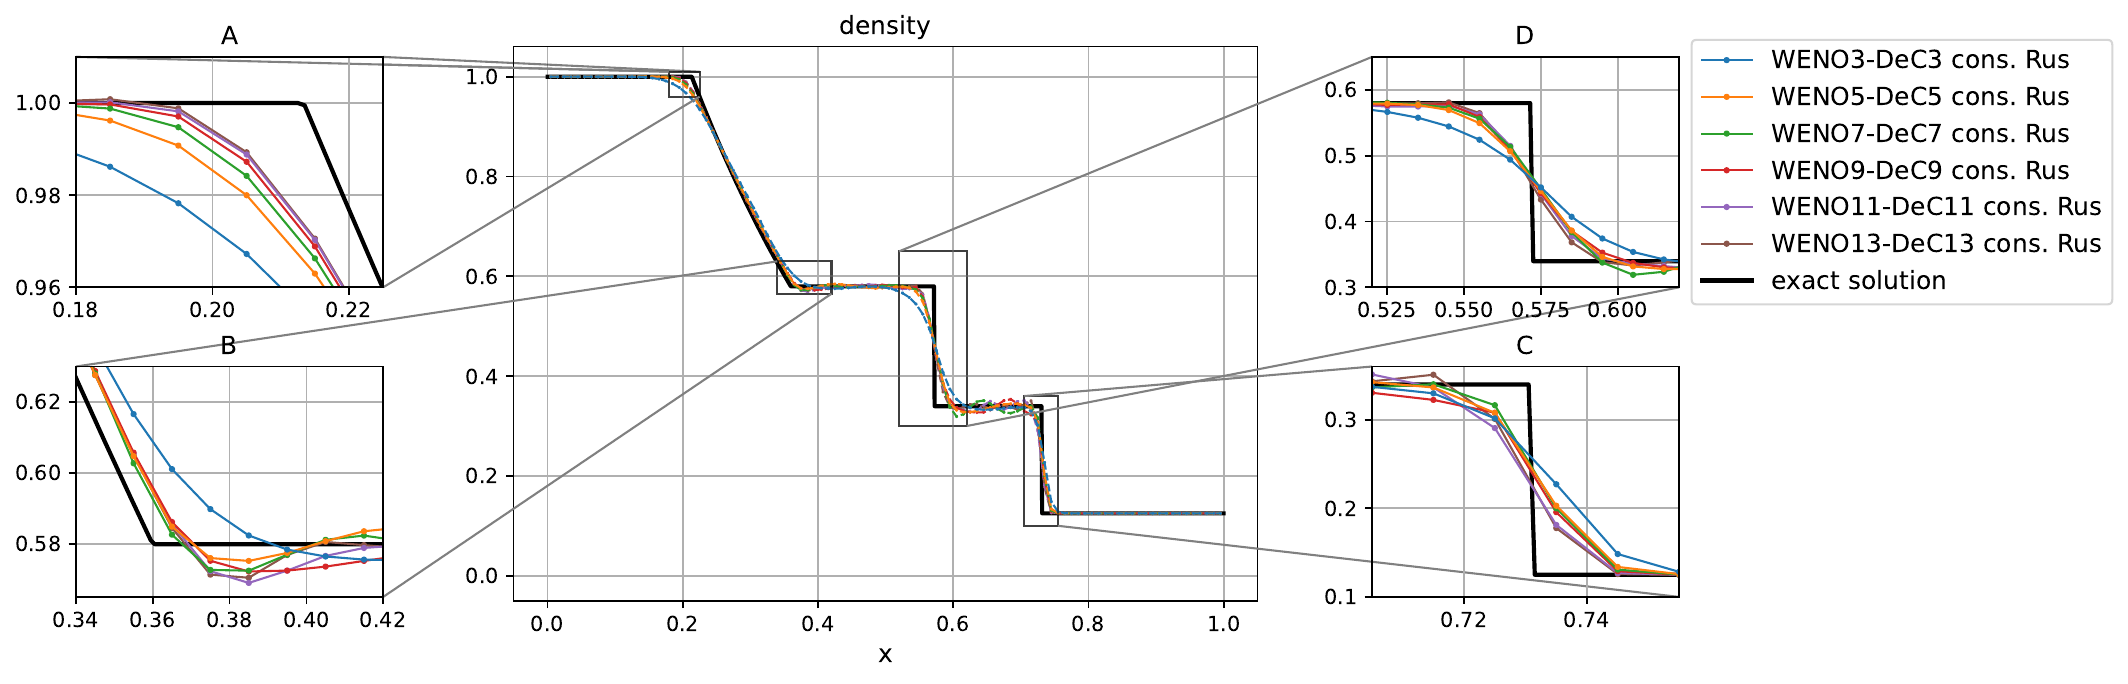}
		\caption{Reconstruction of conserved variables and Rusanov}
	\end{subfigure}
	\\
	\begin{subfigure}[b]{0.8\textwidth}
		\centering
		\includegraphics[width=\textwidth]{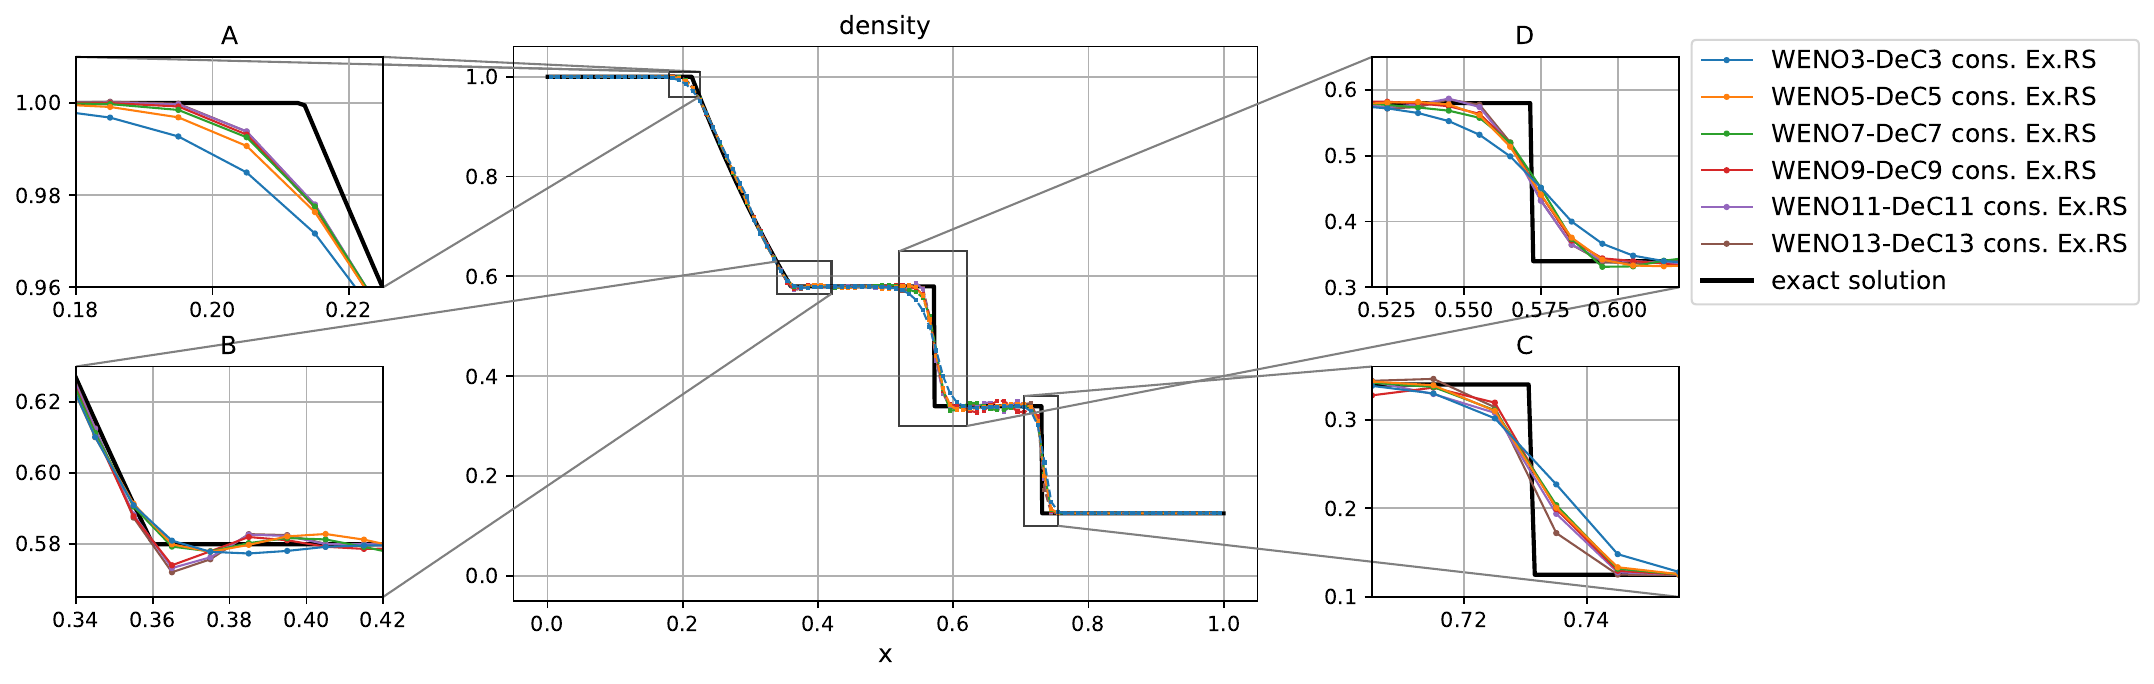}
		\caption{Reconstruction of conserved variables and exact Riemann solver}
	\end{subfigure}
	\\
	\begin{subfigure}[b]{0.8\textwidth}
		\centering
		\includegraphics[width=\textwidth]{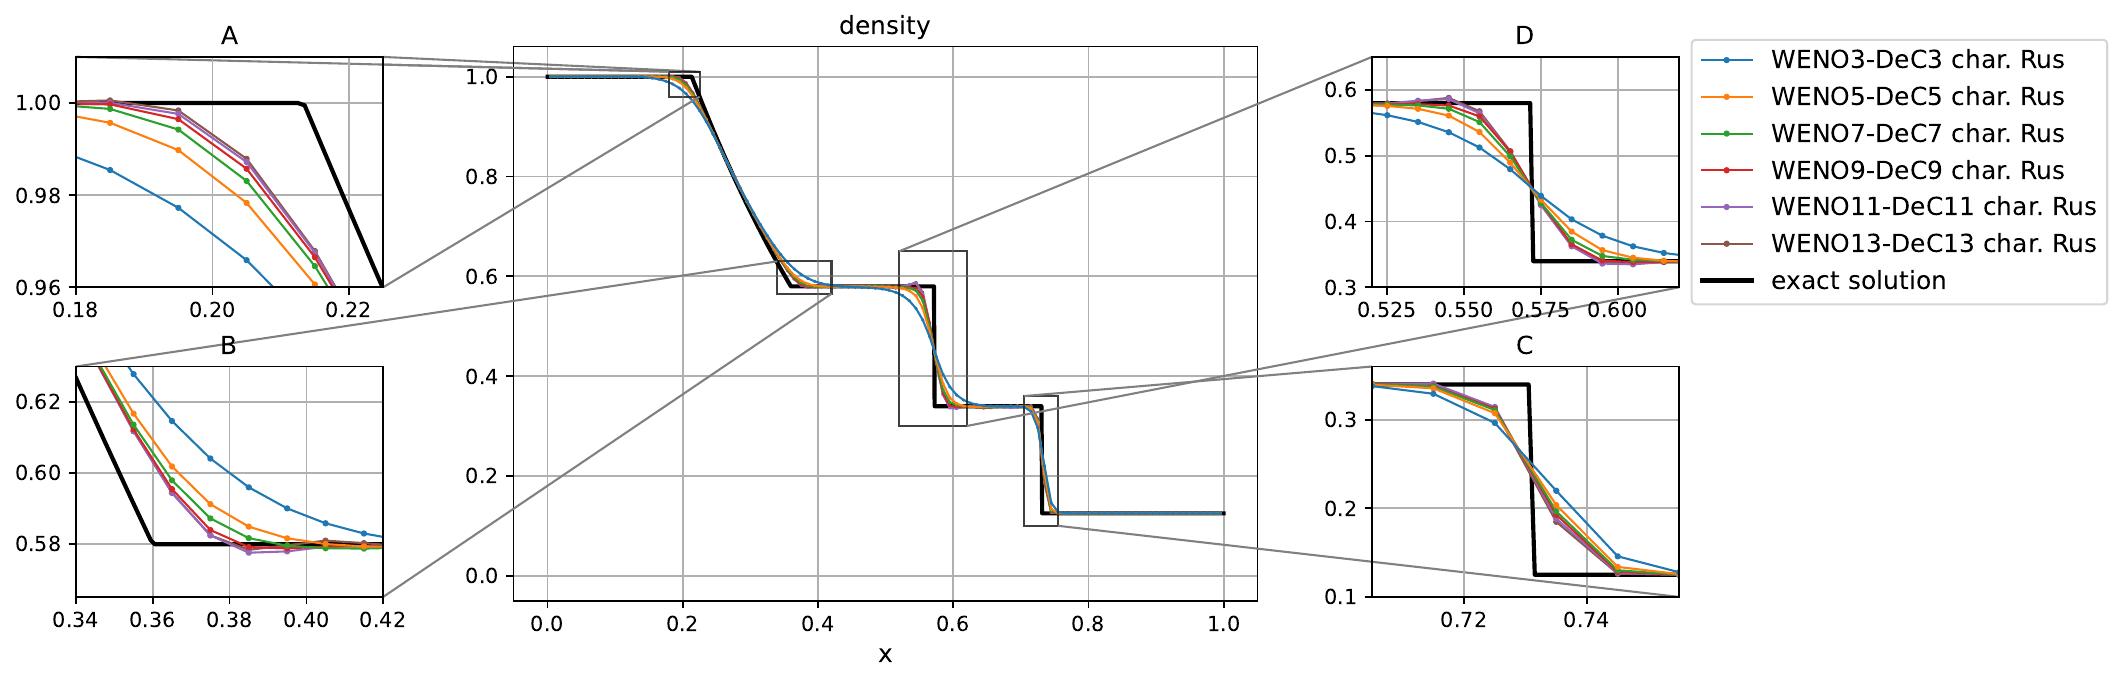}
		\caption{Reconstruction of characteristic variables and Rusanov}
	\end{subfigure}
	\\
	\begin{subfigure}[b]{0.8\textwidth}
		\centering
		\includegraphics[width=\textwidth]{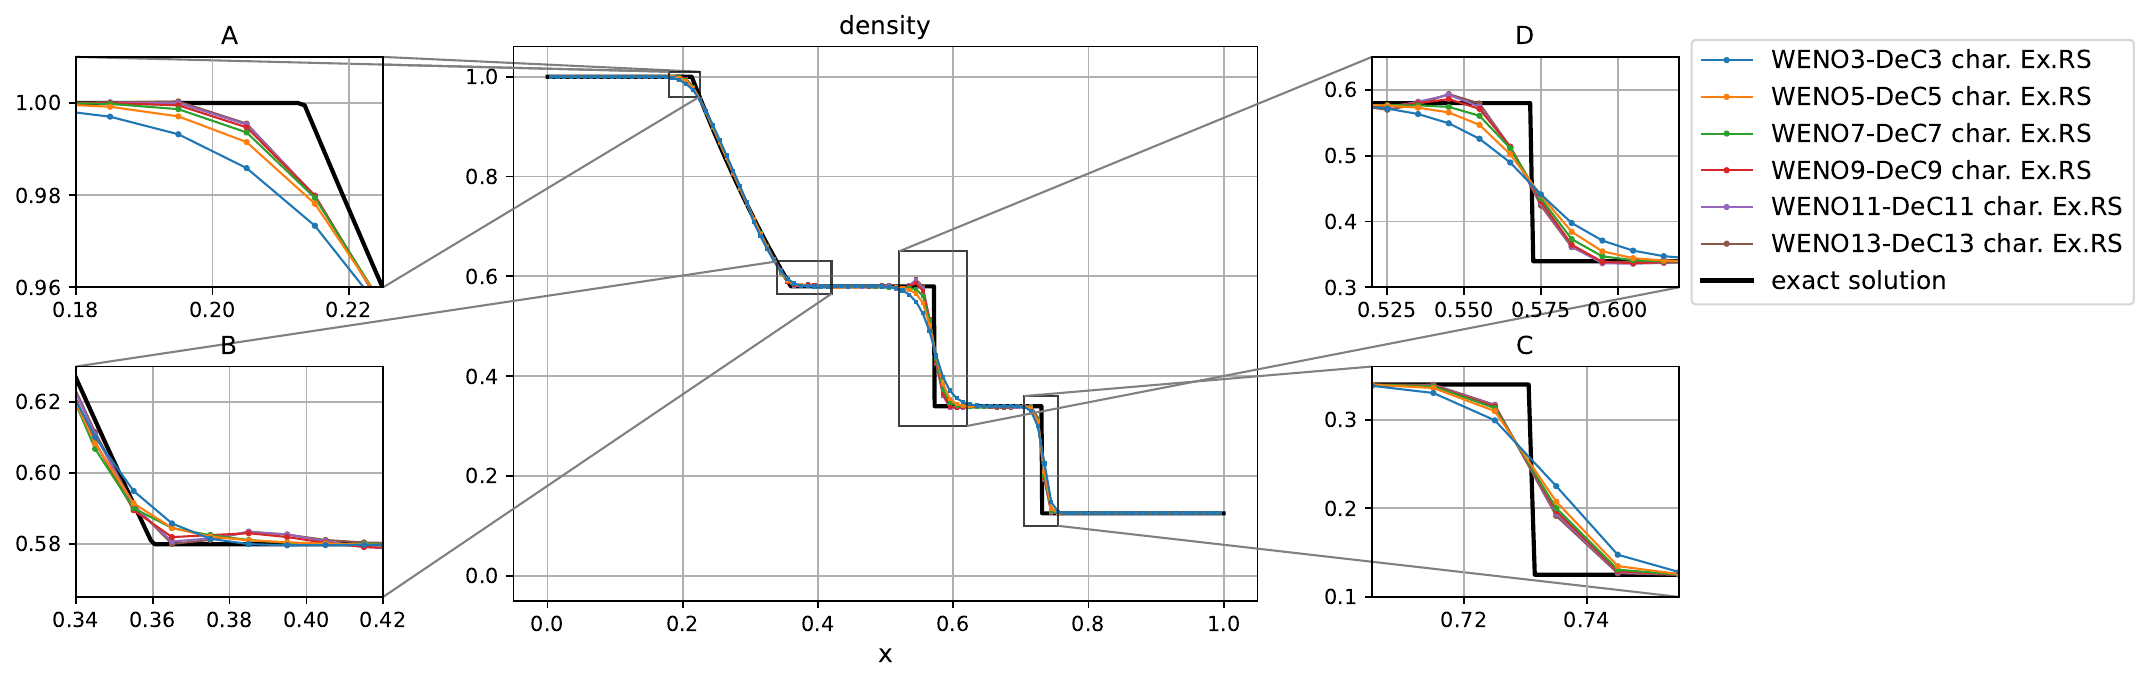}
		\caption{Reconstruction of characteristic variables and exact Riemann solver}
	\end{subfigure}
	\caption{Euler equations, Riemann problem 1: Results for the density obtained through WENO--DeC with $C_{CFL}:=0.95$}
	\label{fig:Euler_1d_RP1_zoom_density}
\end{figure}

\section{Riemann problem 2 (Double rarefaction)}\label{sec:Euler_1d_RP2}
In Figure~\ref{fig:Euler_1d_RP2_relaxed_zoom_density}, we report the results obtained for the density for all settings on th relaxed version of Riemann problem 2 with $C_{CFL}:=0.45$.

\begin{figure}[htbp]
	\centering
	\begin{subfigure}[b]{0.8\textwidth}
		\centering
		\includegraphics[width=\textwidth]{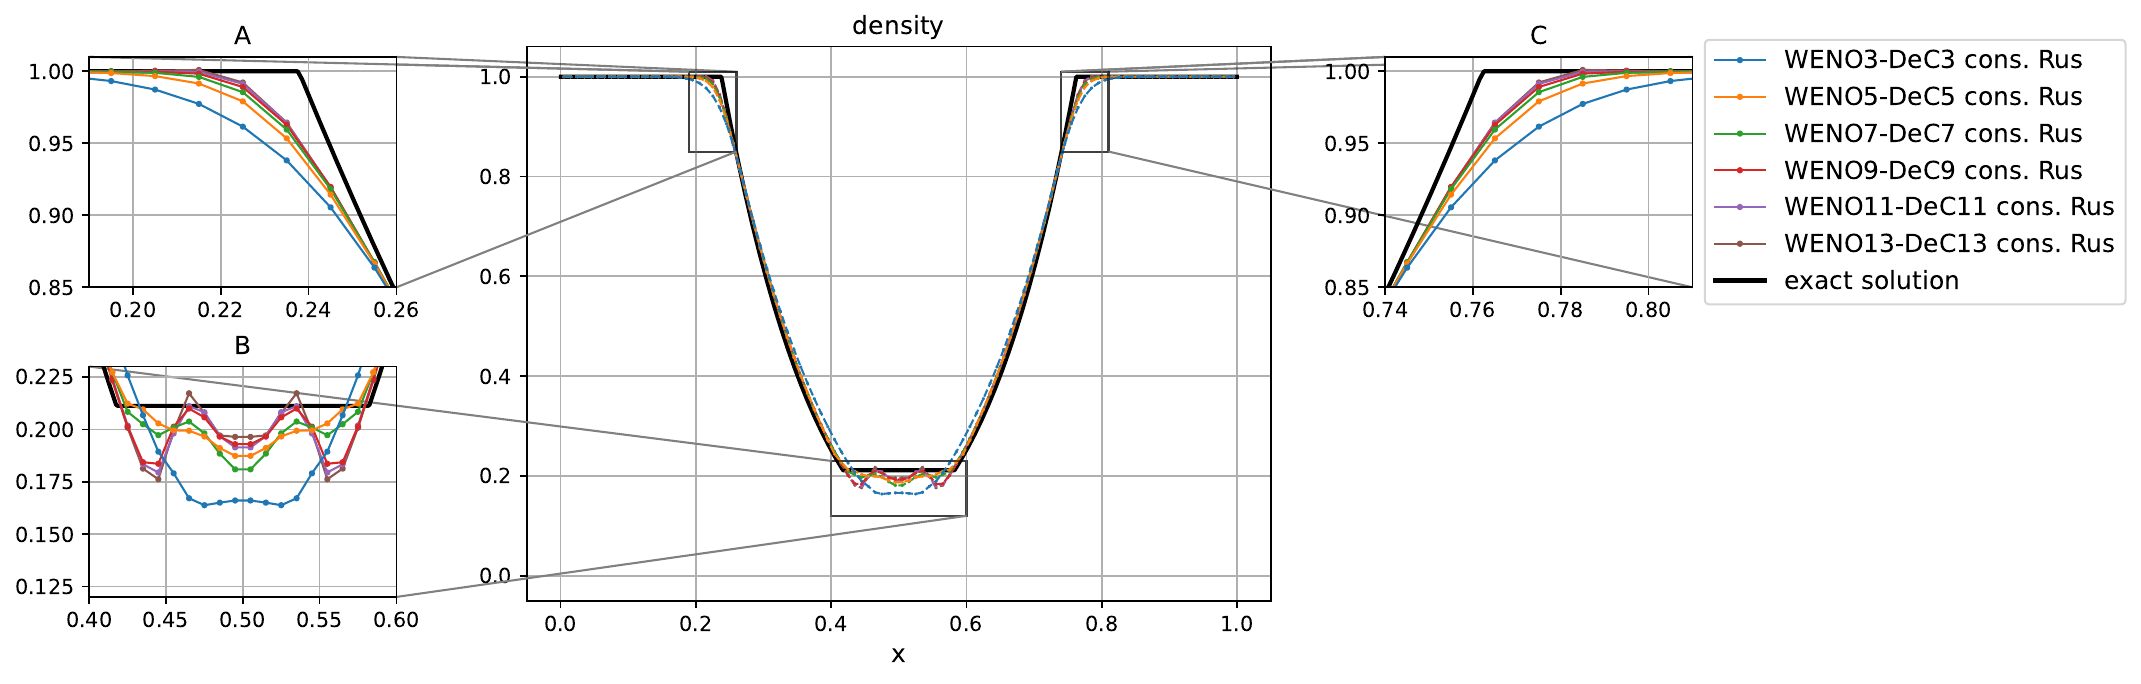}
		\caption{Reconstruction of conserved variables and Rusanov}
	\end{subfigure}
	\\
	\begin{subfigure}[b]{0.8\textwidth}
		\centering
		\includegraphics[width=\textwidth]{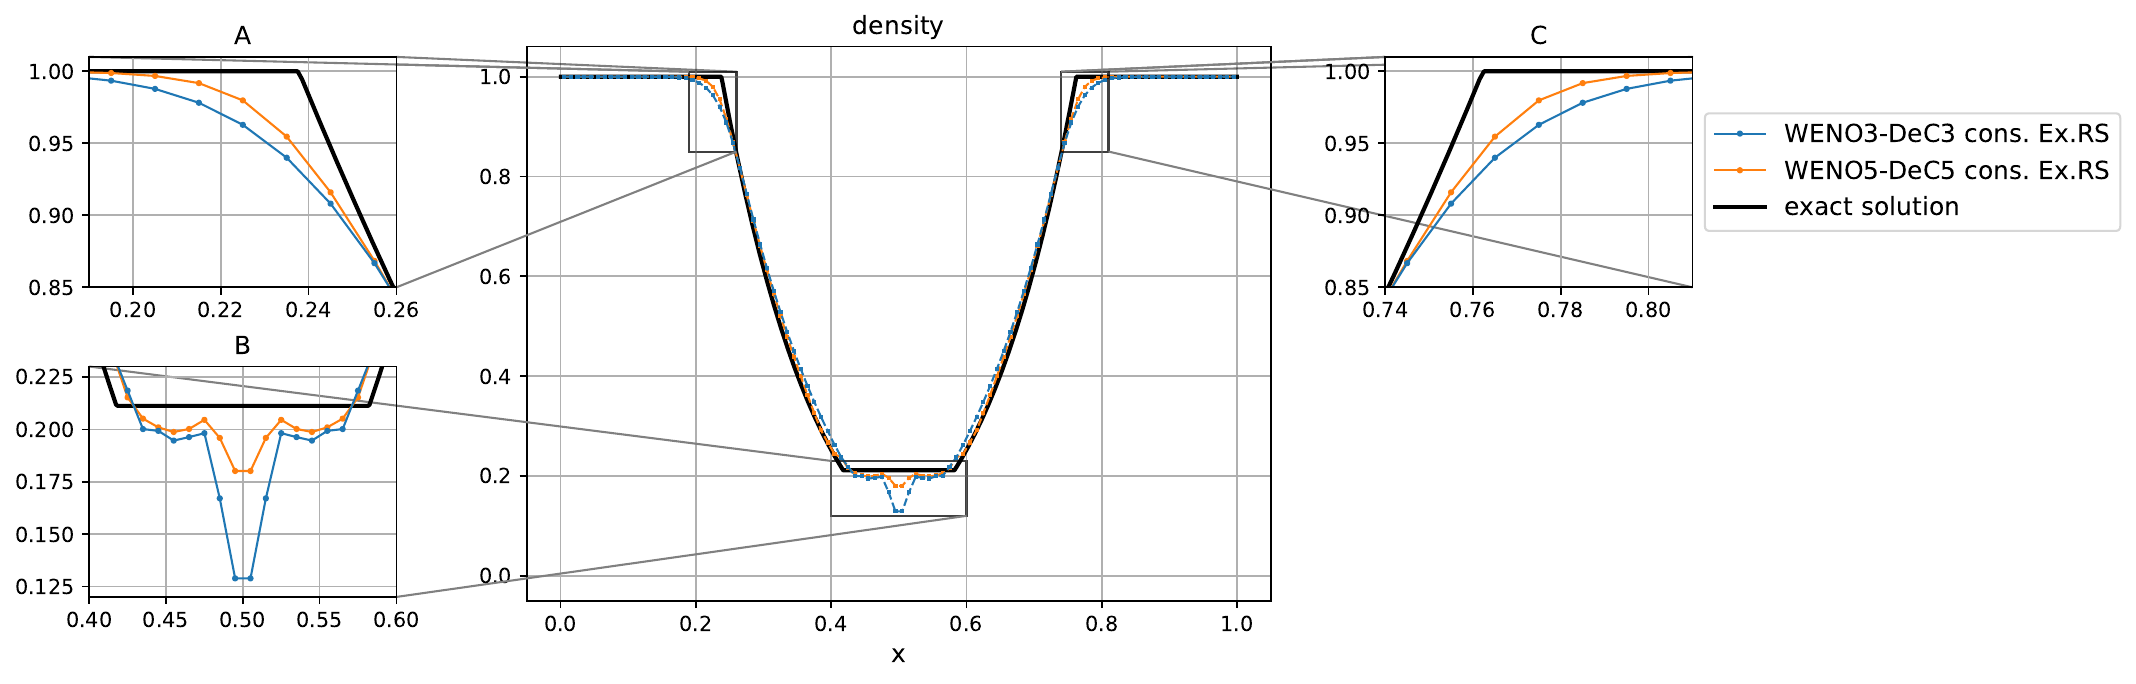}
		\caption{Reconstruction of conserved variables and exact Riemann solver}
	\end{subfigure}
	\\
	\begin{subfigure}[b]{0.8\textwidth}
		\centering
		\includegraphics[width=\textwidth]{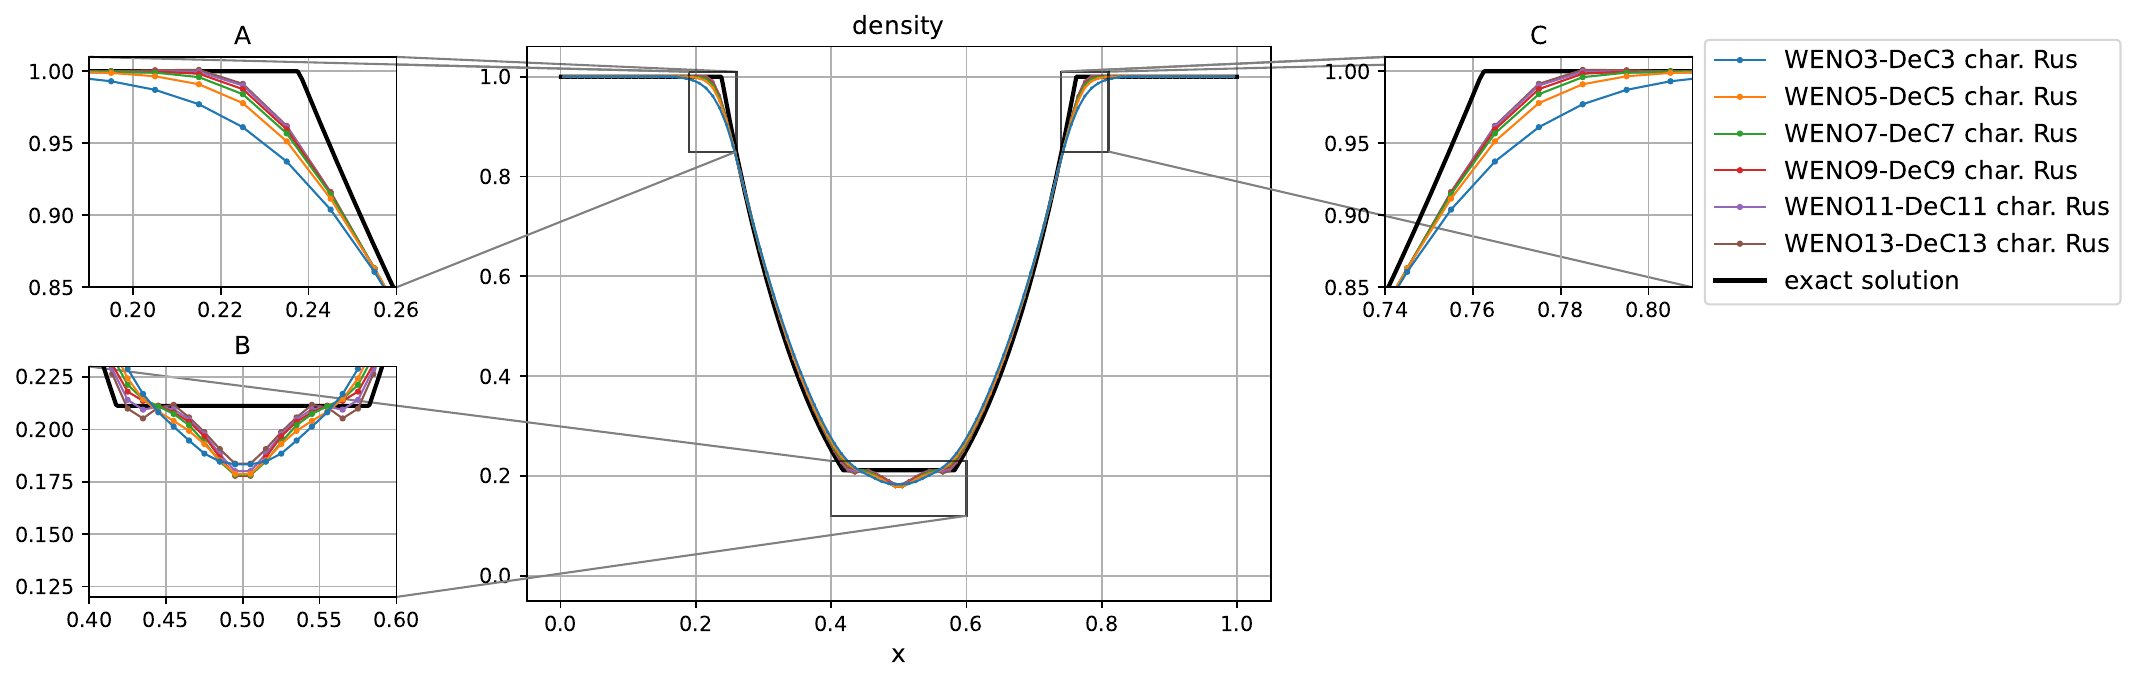}
		\caption{Reconstruction of characteristic variables and Rusanov}
	\end{subfigure}
	\\
	\begin{subfigure}[b]{0.8\textwidth}
		\centering
		\includegraphics[width=\textwidth]{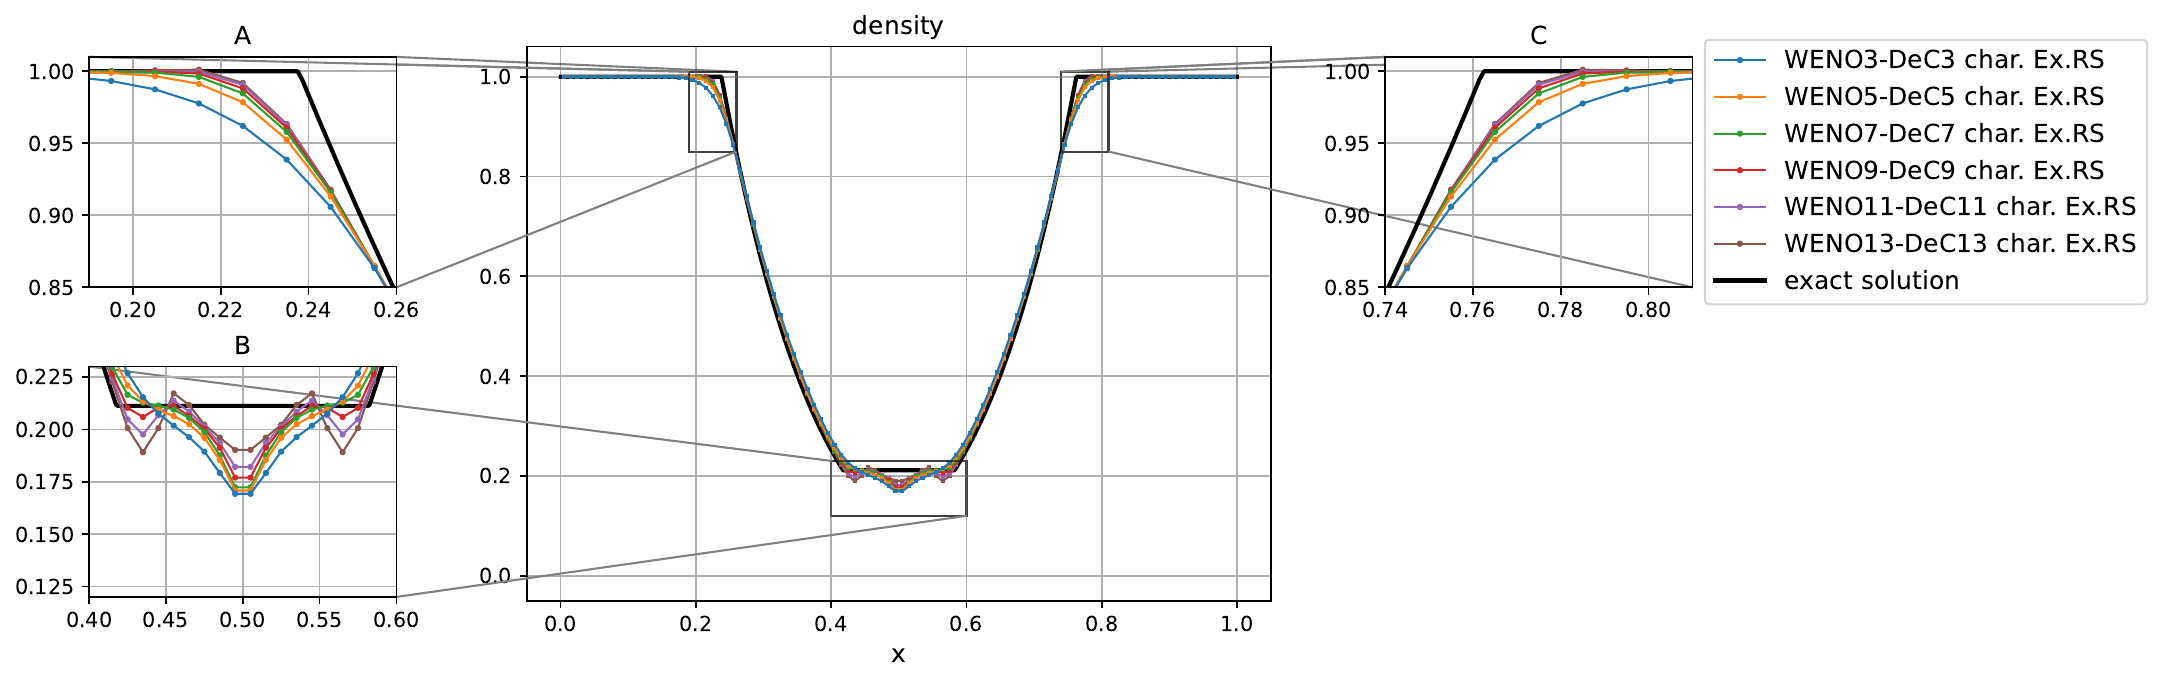}
		\caption{Reconstruction of characteristic variables and exact Riemann solver}
	\end{subfigure}
	\caption{Euler equations, relaxed Riemann problem 2: Results for the density obtained through WENO--DeC with $C_{CFL}:=0.45$}
	\label{fig:Euler_1d_RP2_relaxed_zoom_density}
\end{figure}

\section{Riemann problem 3 (Left Woodward--Colella)}\label{sec:Euler_1d_RP3}
In Figure~\ref{fig:Euler_1d_RP3_zoom_density}, we report the results obtained for the density for all settings on Riemann problem 3 with $C_{CFL}:=0.45$.

\begin{figure}[htbp]
	\centering
	\begin{subfigure}[b]{0.45\textwidth}
		\centering
		\includegraphics[width=\textwidth]{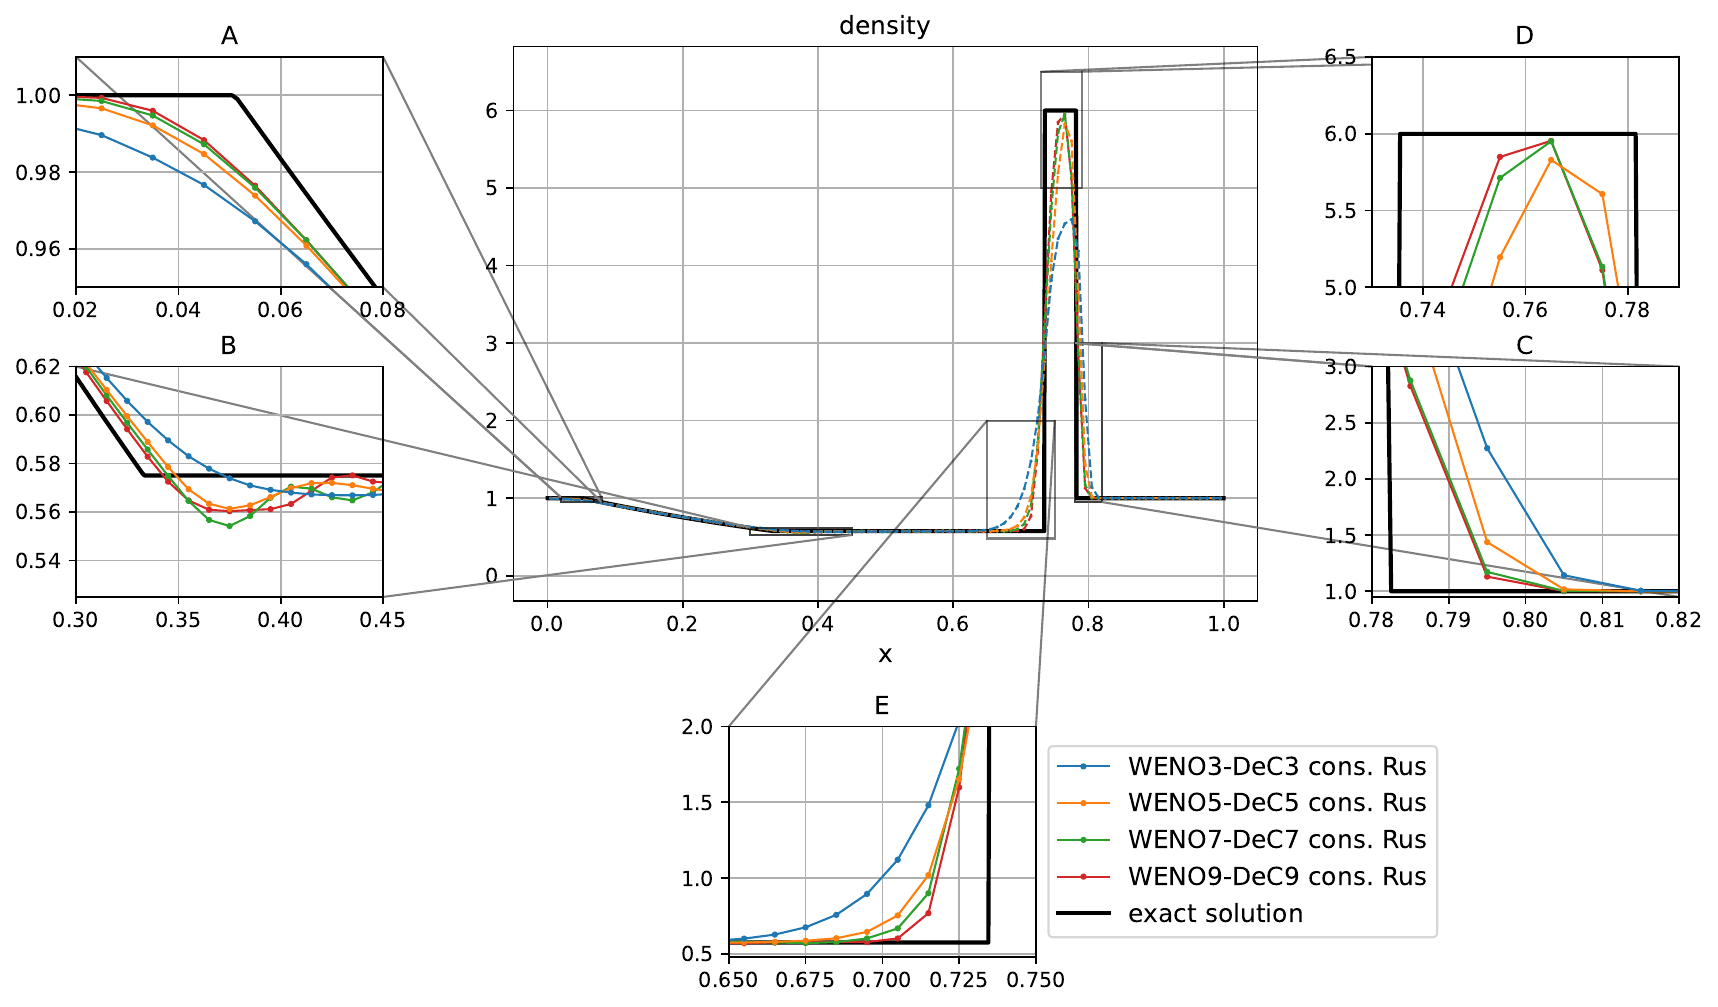}
		\caption{Reconstruction of conserved variables and Rusanov}
	\end{subfigure}
	\hfill
	\begin{subfigure}[b]{0.45\textwidth}
		\centering
		\includegraphics[width=\textwidth]{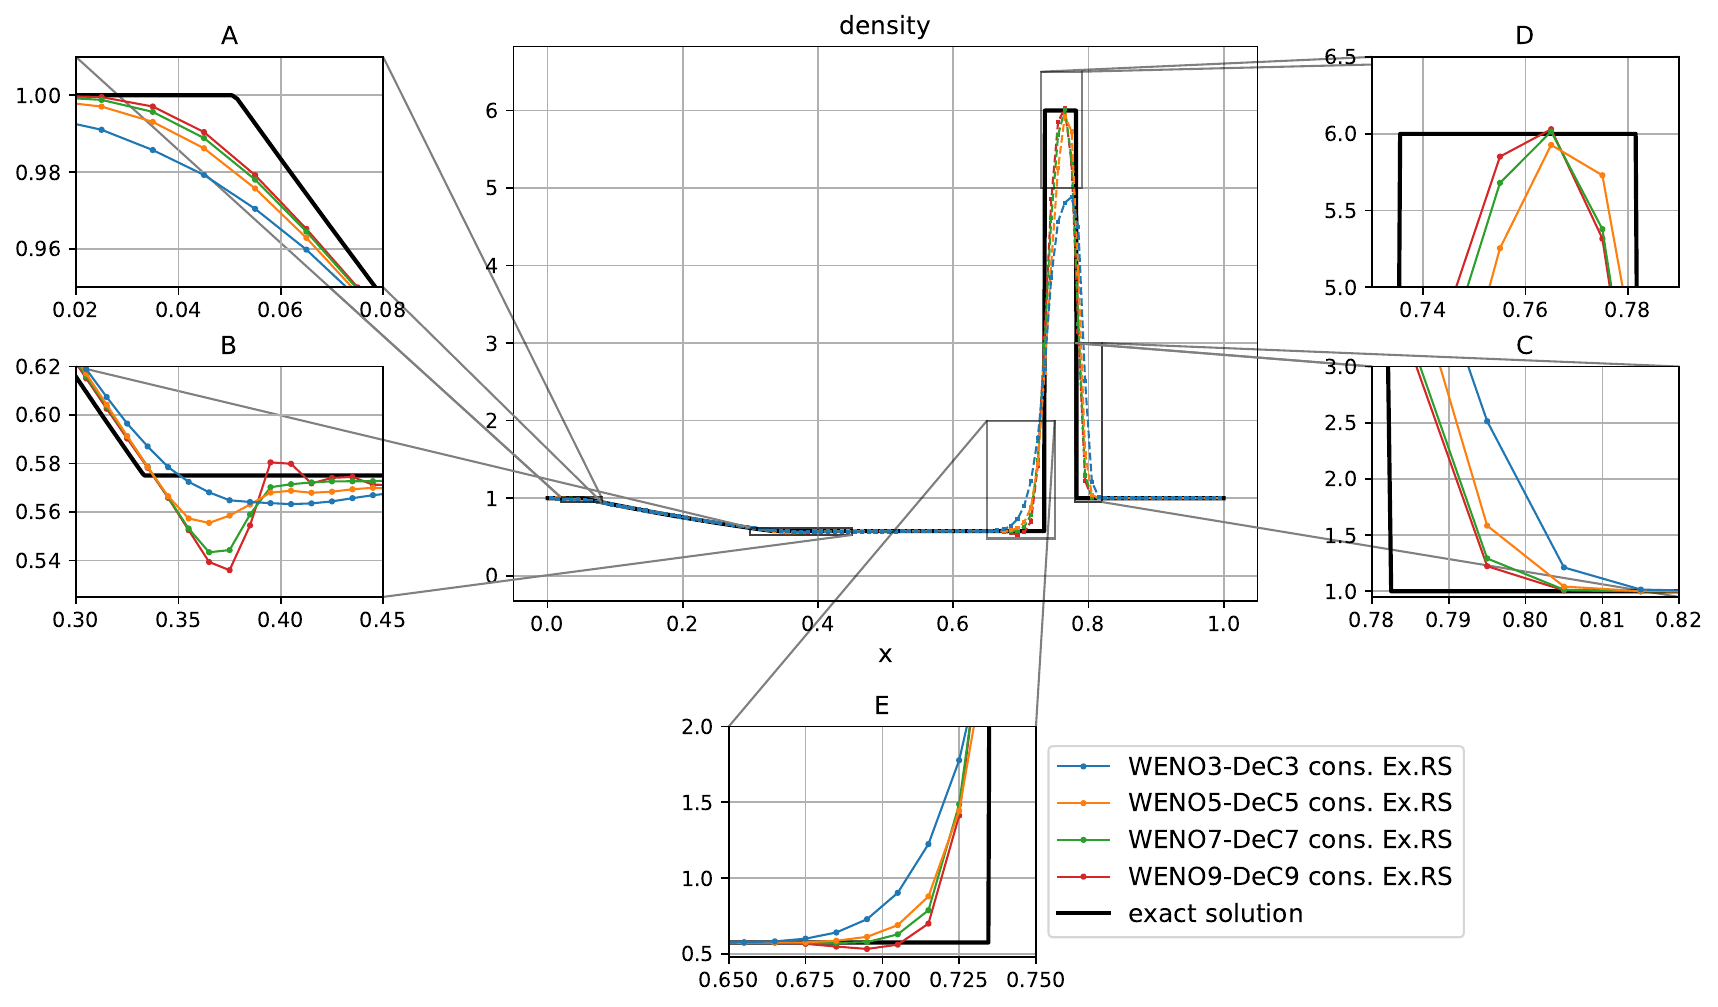}
		\caption{Reconstruction of conserved variables and exact Riemann solver}
	\end{subfigure}
	\\
	\begin{subfigure}[b]{0.45\textwidth}
		\centering
		\includegraphics[width=\textwidth]{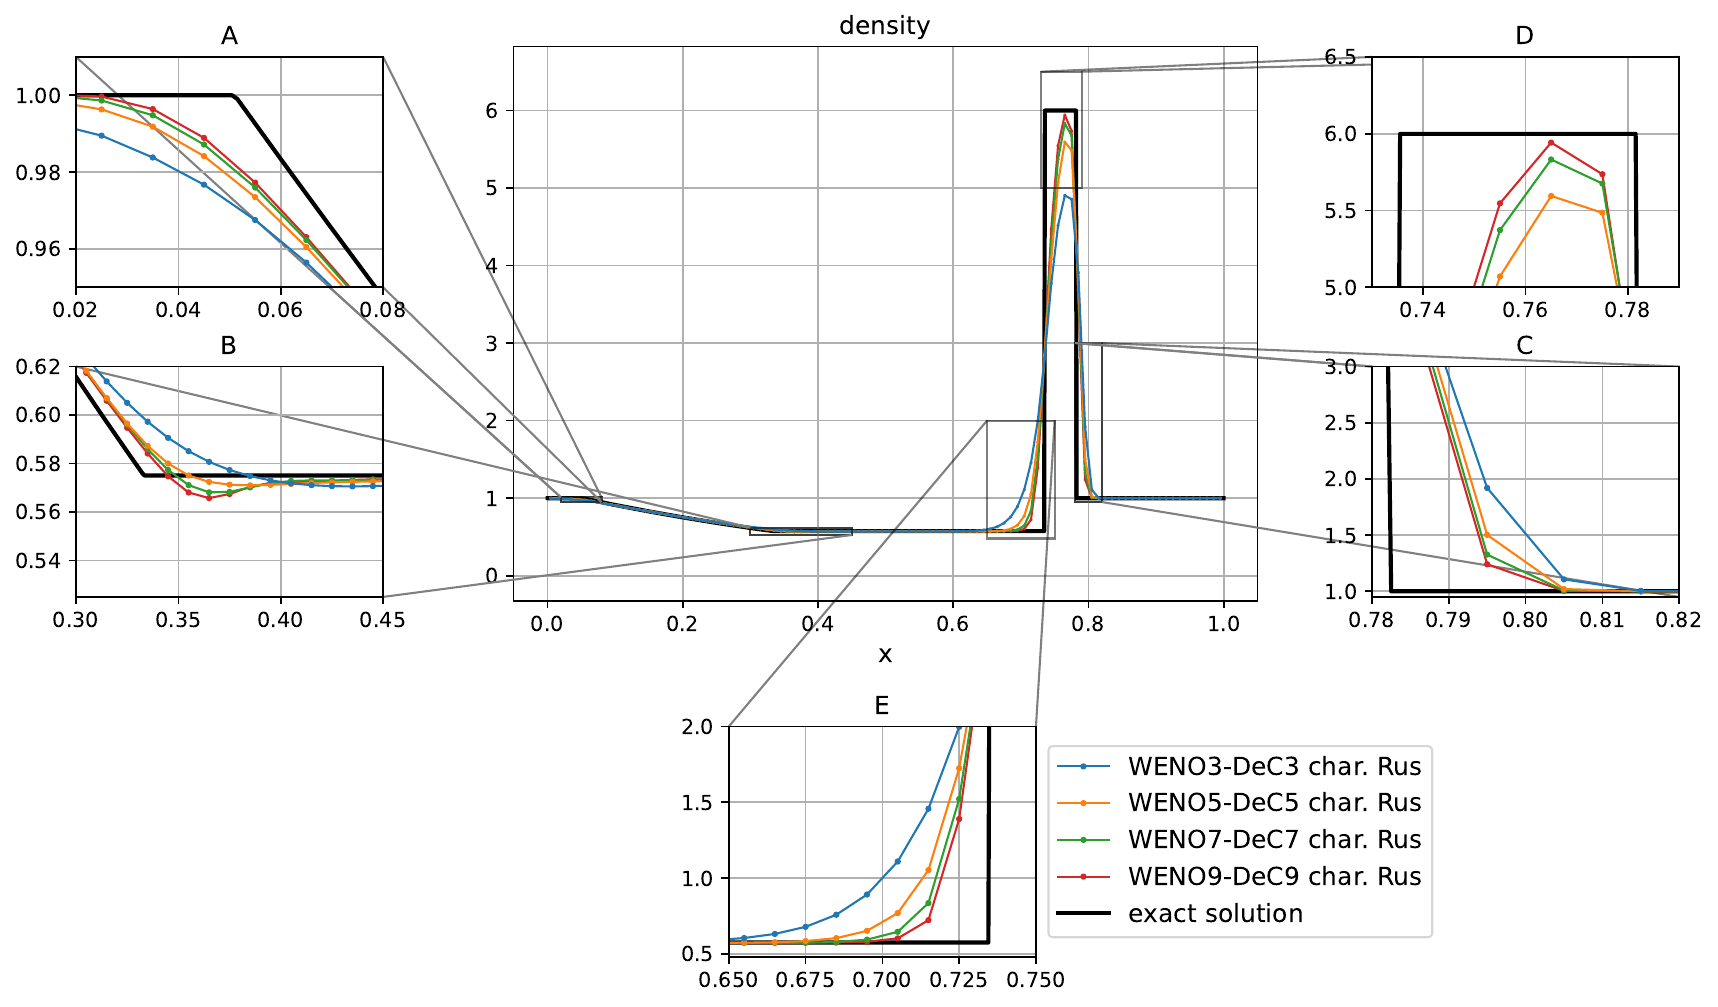}
		\caption{Reconstruction of characteristic variables and Rusanov}
	\end{subfigure}
	\hfill
	\begin{subfigure}[b]{0.45\textwidth}
		\centering
		\includegraphics[width=\textwidth]{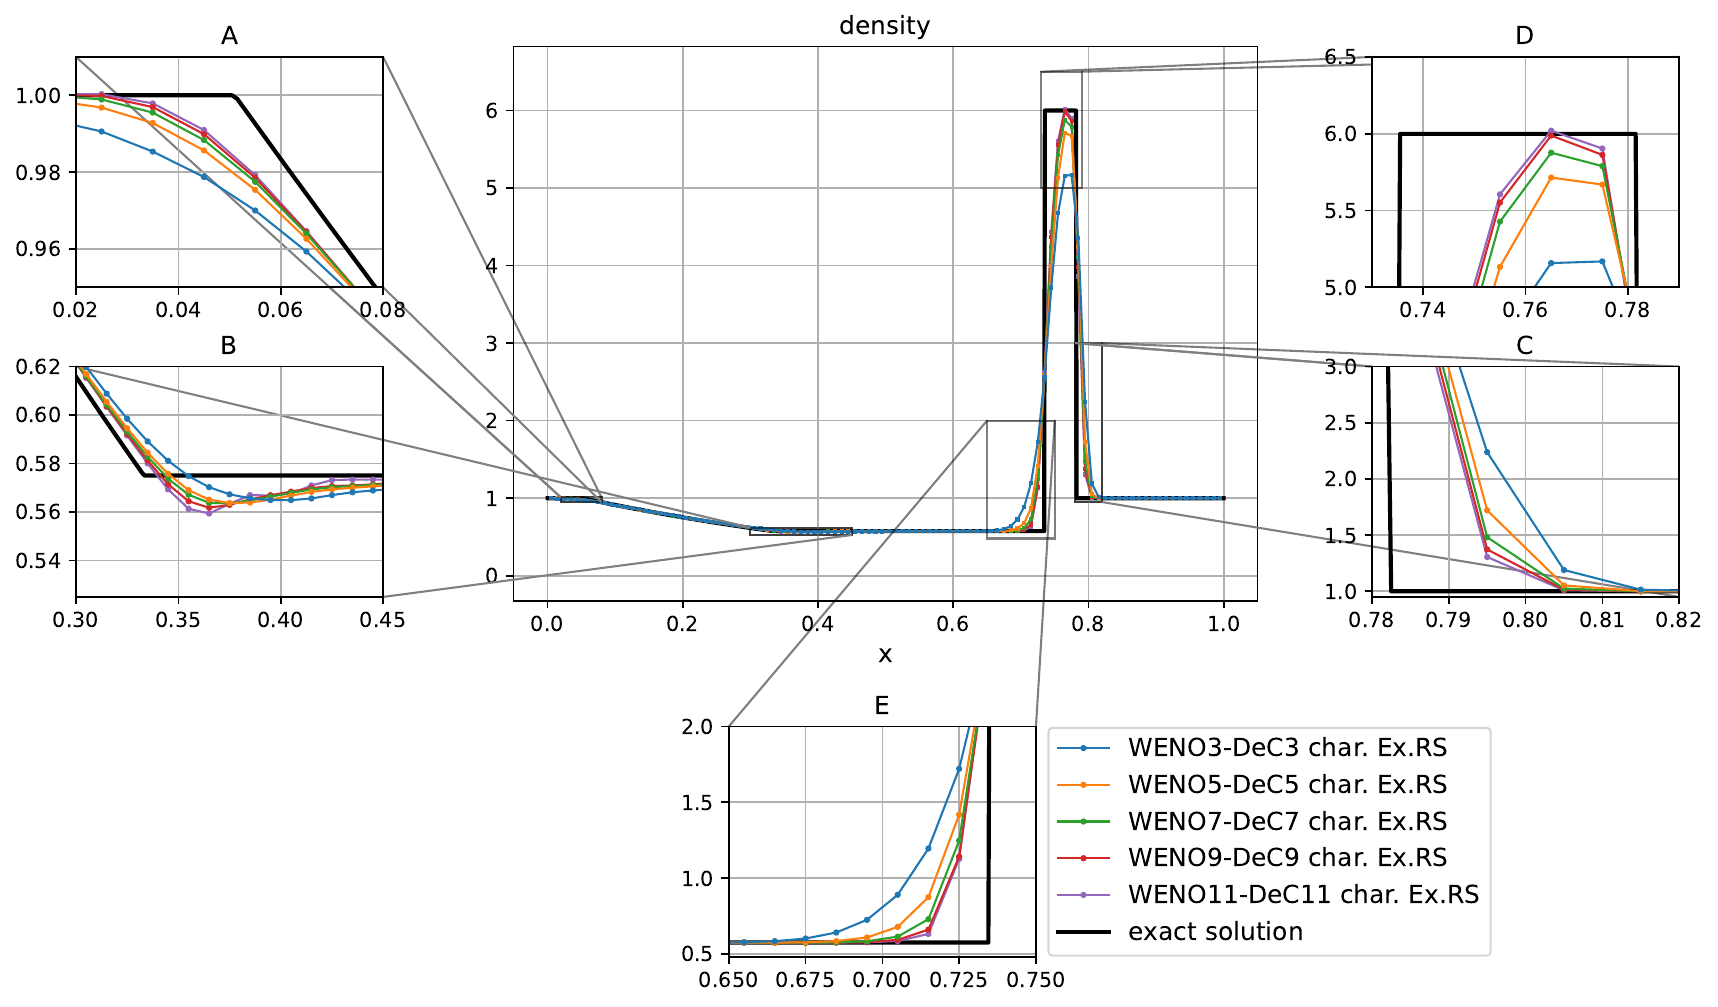}
		\caption{Reconstruction of characteristic variables and exact Riemann solver}
	\end{subfigure}
	\caption{Euler equations, Riemann problem 3: Results for the density obtained through WENO--DeC with $C_{CFL}:=0.45$}
	\label{fig:Euler_1d_RP3_zoom_density}
\end{figure}

\section{Riemann problem 4 (Collision of two shocks)}\label{sec:Euler_1d_RP4}
In Figure~\ref{fig:Euler_1d_RP4_zoom_density}, we report the results obtained for the density for all settings on Riemann problem 4 with $C_{CFL}:=0.95$.

\begin{figure}[htbp]
	\centering
	\begin{subfigure}[b]{0.8\textwidth}
		\centering
		\includegraphics[width=\textwidth]{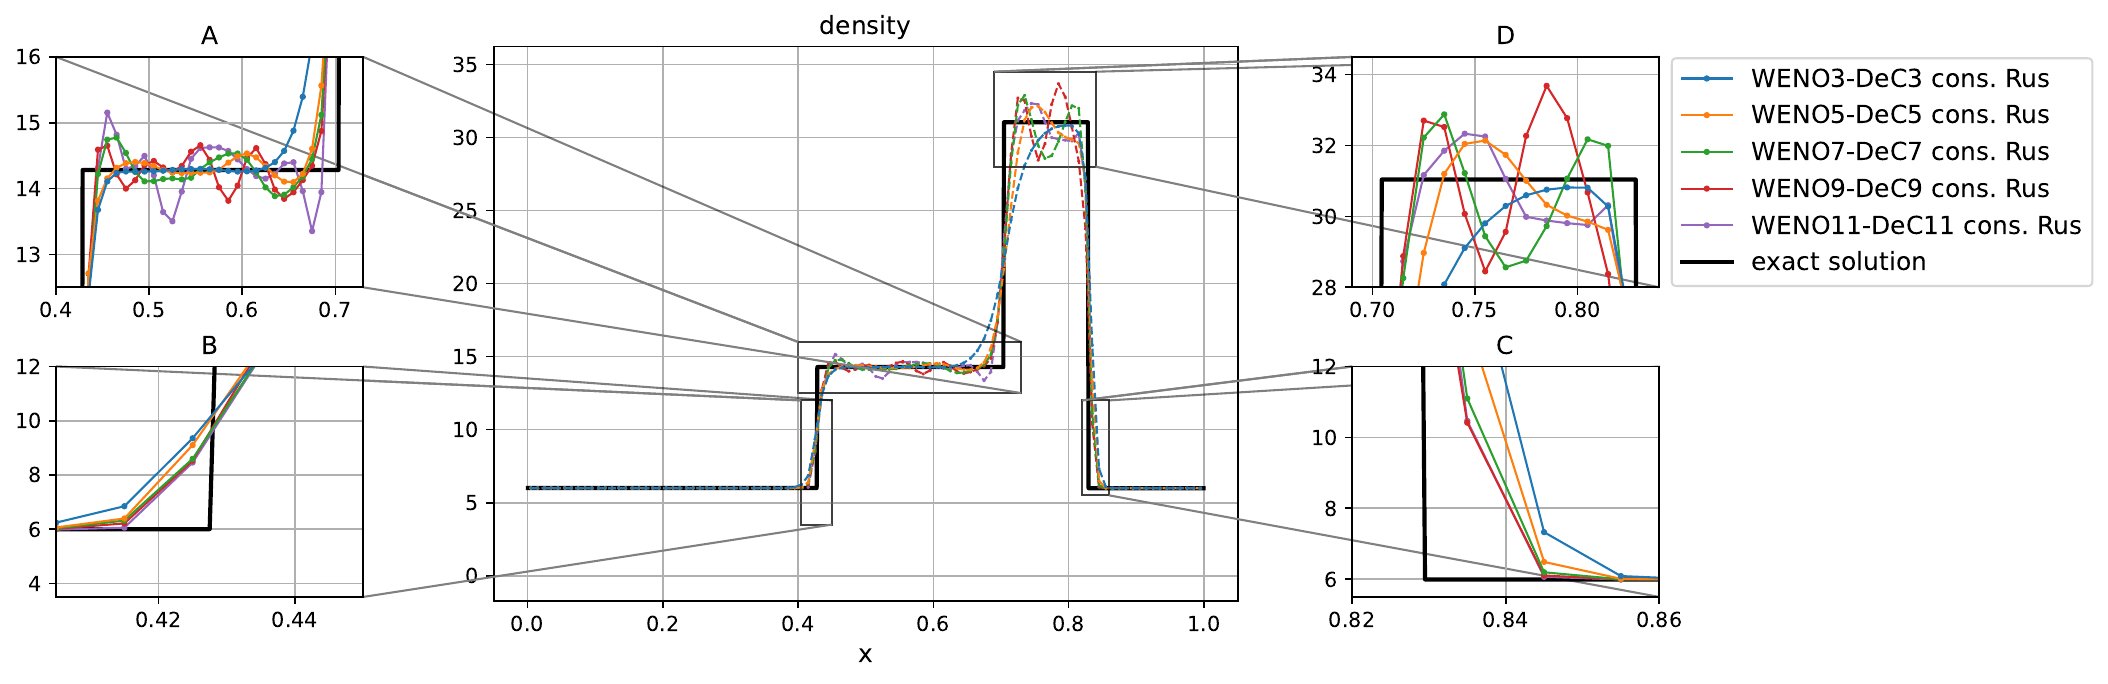}
		\caption{Reconstruction of conserved variables and Rusanov}
	\end{subfigure}
	\\
	\begin{subfigure}[b]{0.8\textwidth}
		\centering
		\includegraphics[width=\textwidth]{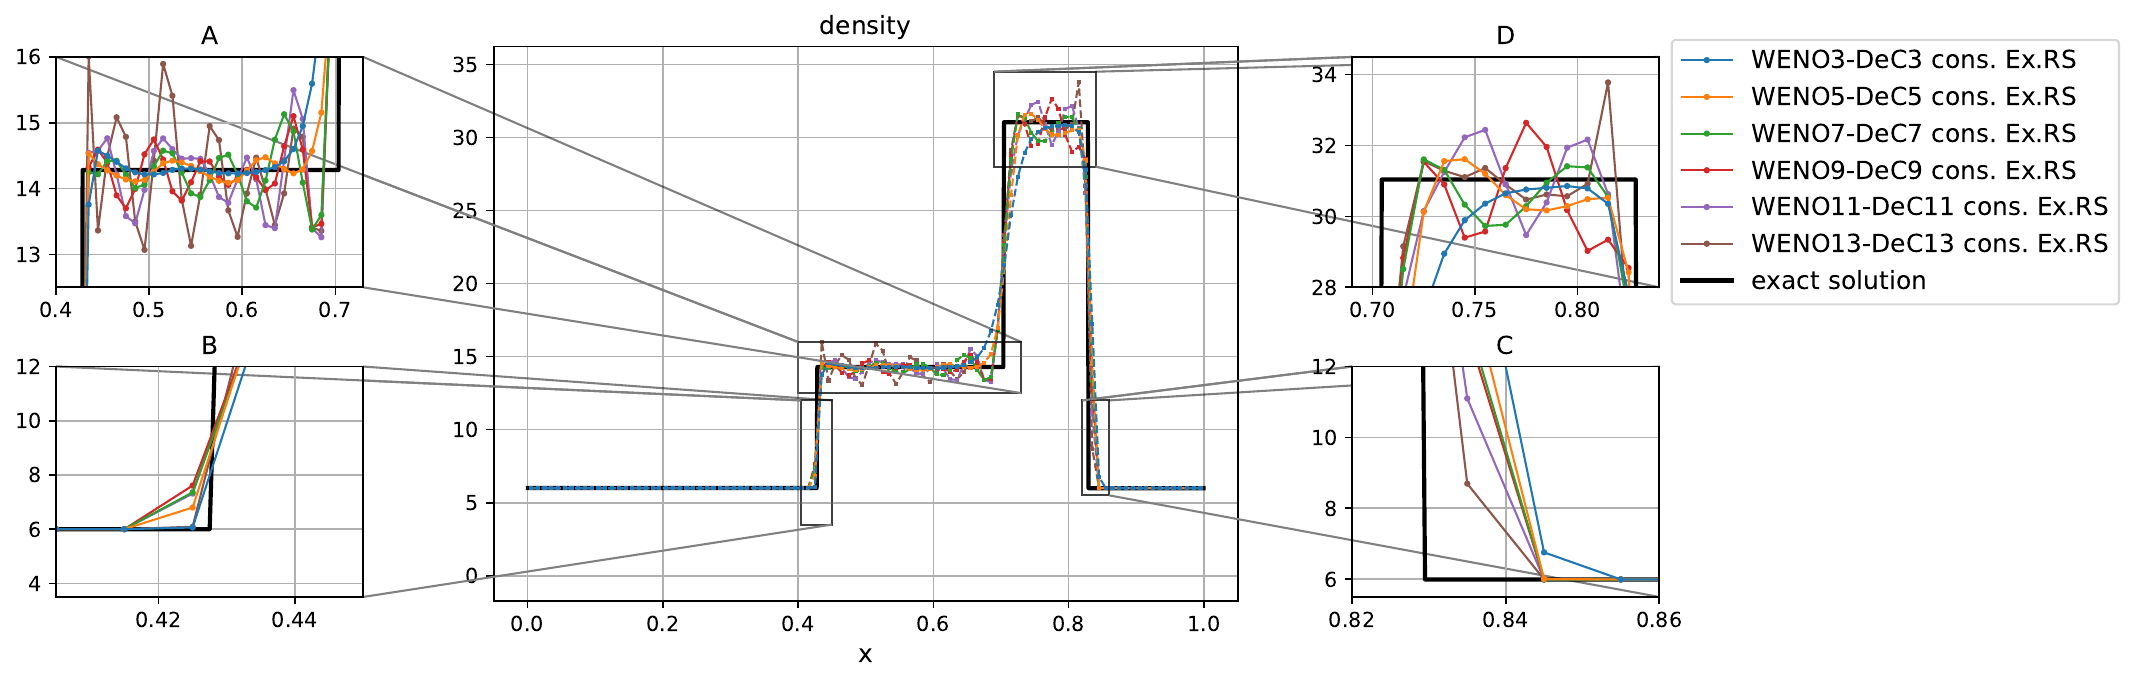}
		\caption{Reconstruction of conserved variables and exact Riemann solver}
	\end{subfigure}
	\\
	\begin{subfigure}[b]{0.8\textwidth}
		\centering
		\includegraphics[width=\textwidth]{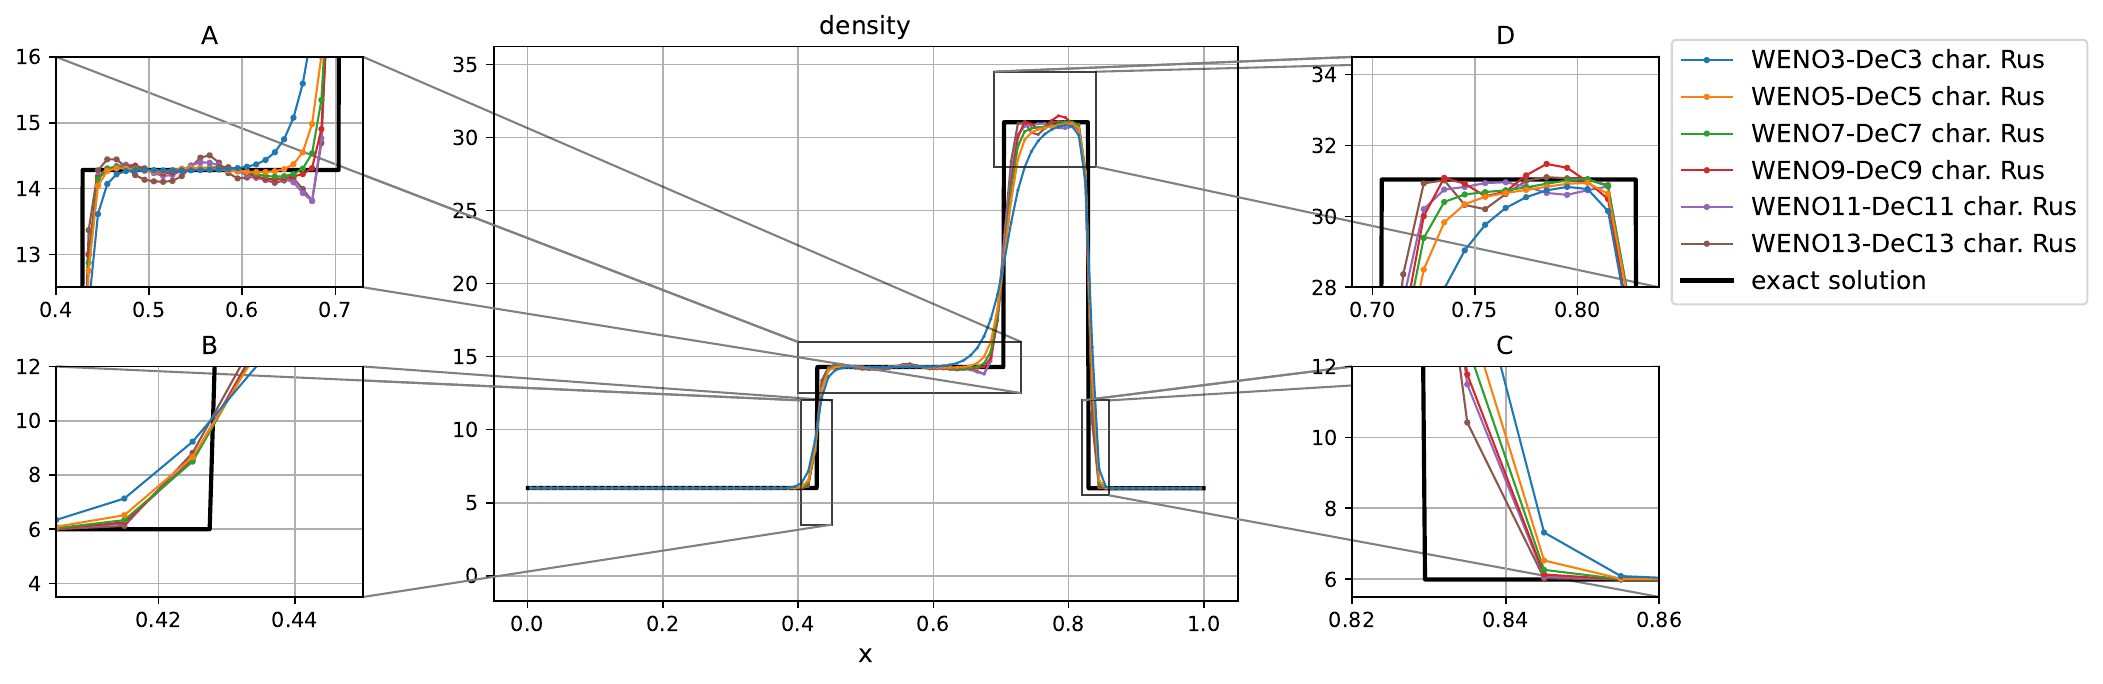}
		\caption{Reconstruction of characteristic variables and Rusanov}
	\end{subfigure}
	\\
	\begin{subfigure}[b]{0.8\textwidth}
		\centering
		\includegraphics[width=\textwidth]{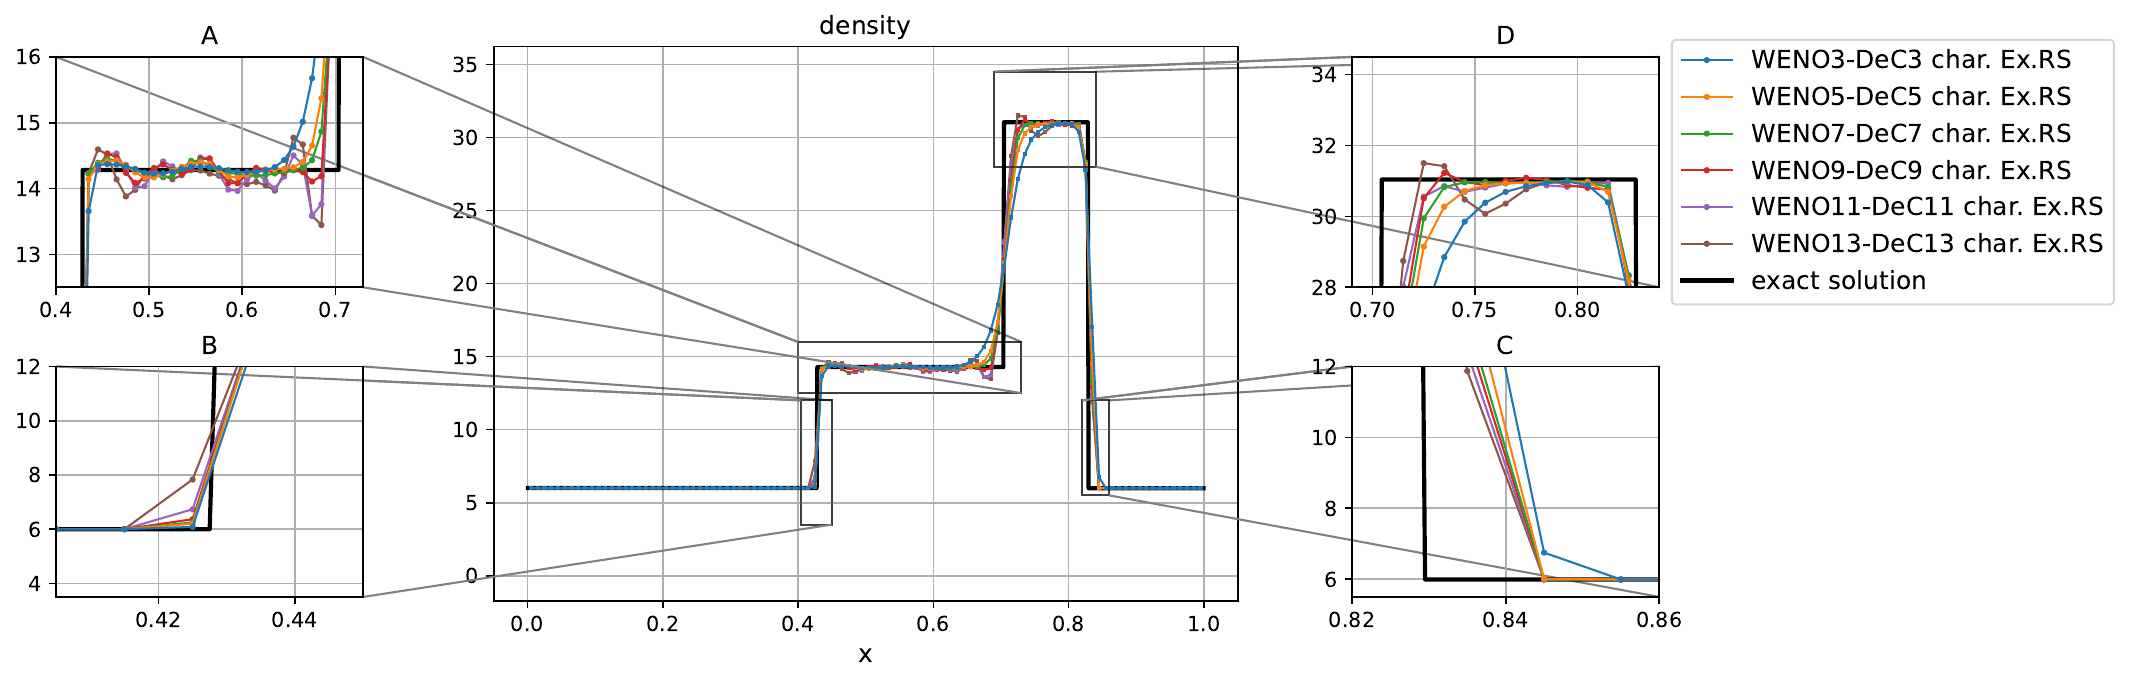}
		\caption{Reconstruction of characteristic variables and exact Riemann solver}
	\end{subfigure}
	\caption{Euler equations, Riemann problem 4: Results for the density obtained through WENO--DeC with $C_{CFL}:=0.95$}
	\label{fig:Euler_1d_RP4_zoom_density}
\end{figure}

\section{Riemann problem 5 (Stationary contact)}\label{sec:Euler_1d_RP5}
In Figure~\ref{fig:Euler_1d_RP5_zoom_density}, we report the results obtained for the density for all settings on Riemann problem 5 with $C_{CFL}:=0.1$.
Let us notice that all simulations with reconstruction of conserved variables and Rusanov for any order crashed. Hence, the related results are missing.

\begin{figure}[htbp]
	\centering
	\begin{subfigure}[b]{0.6\textwidth}
		\centering
		\includegraphics[width=\textwidth]{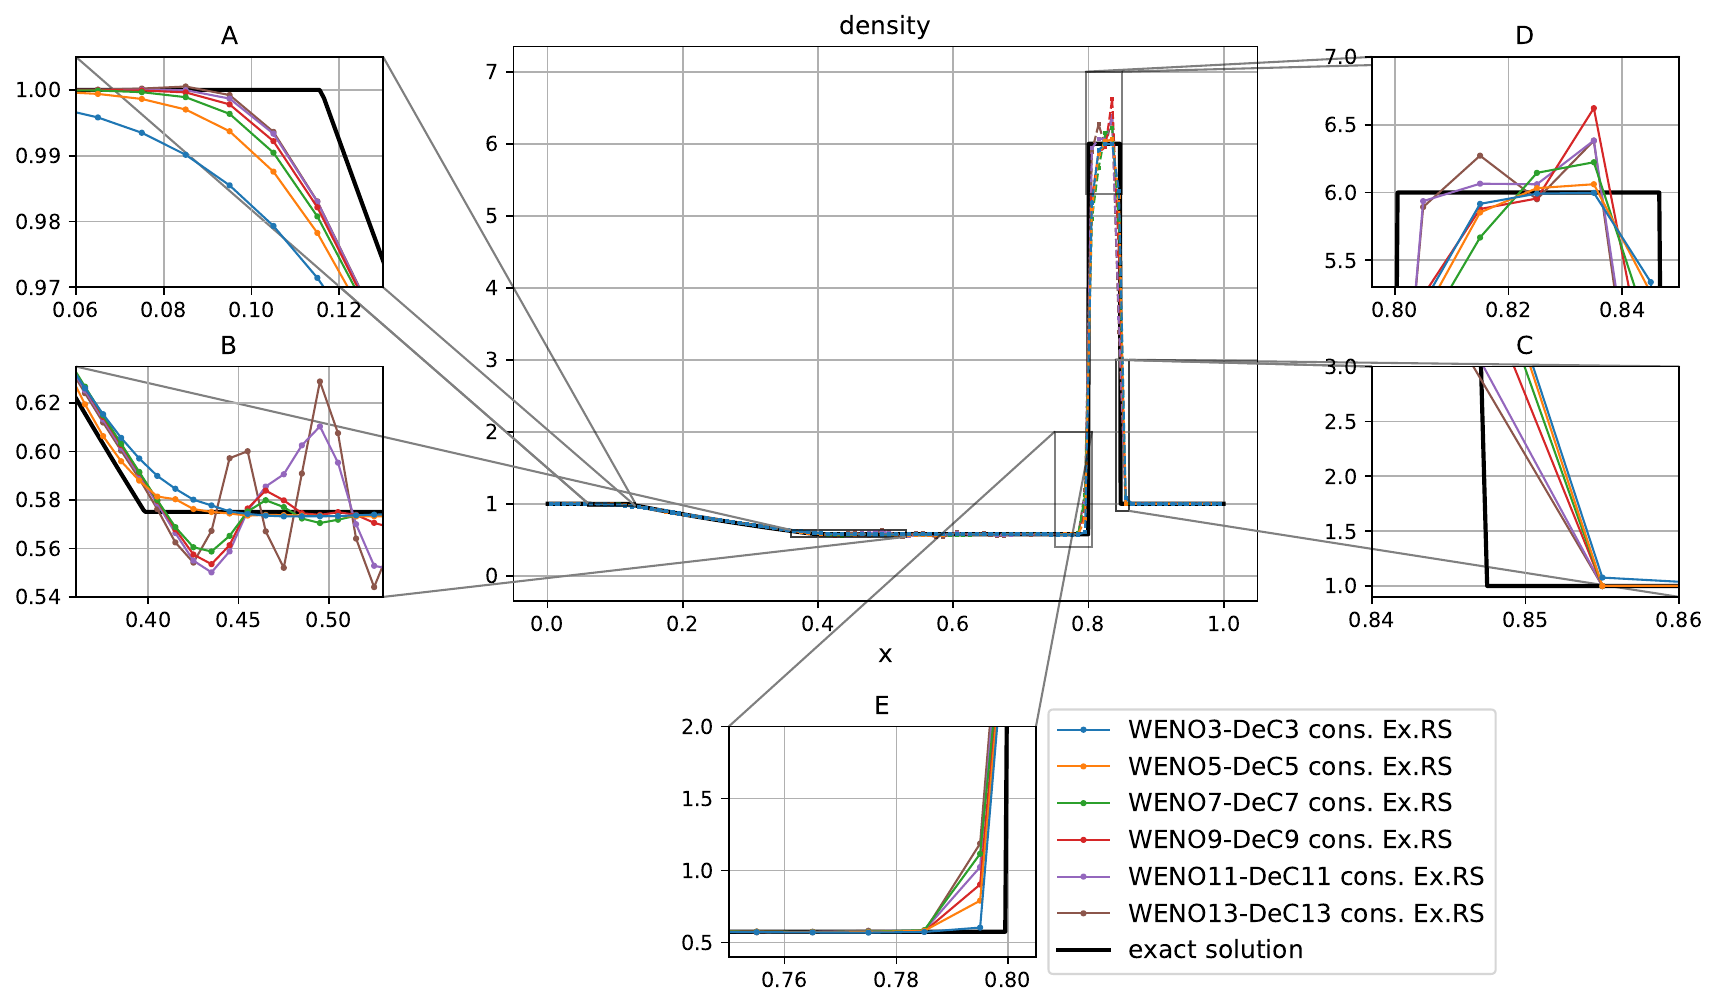}
		\caption{Reconstruction of conserved variables and exact Riemann solver}
	\end{subfigure}
	\\
	\begin{subfigure}[b]{0.6\textwidth}
		\centering
		\includegraphics[width=\textwidth]{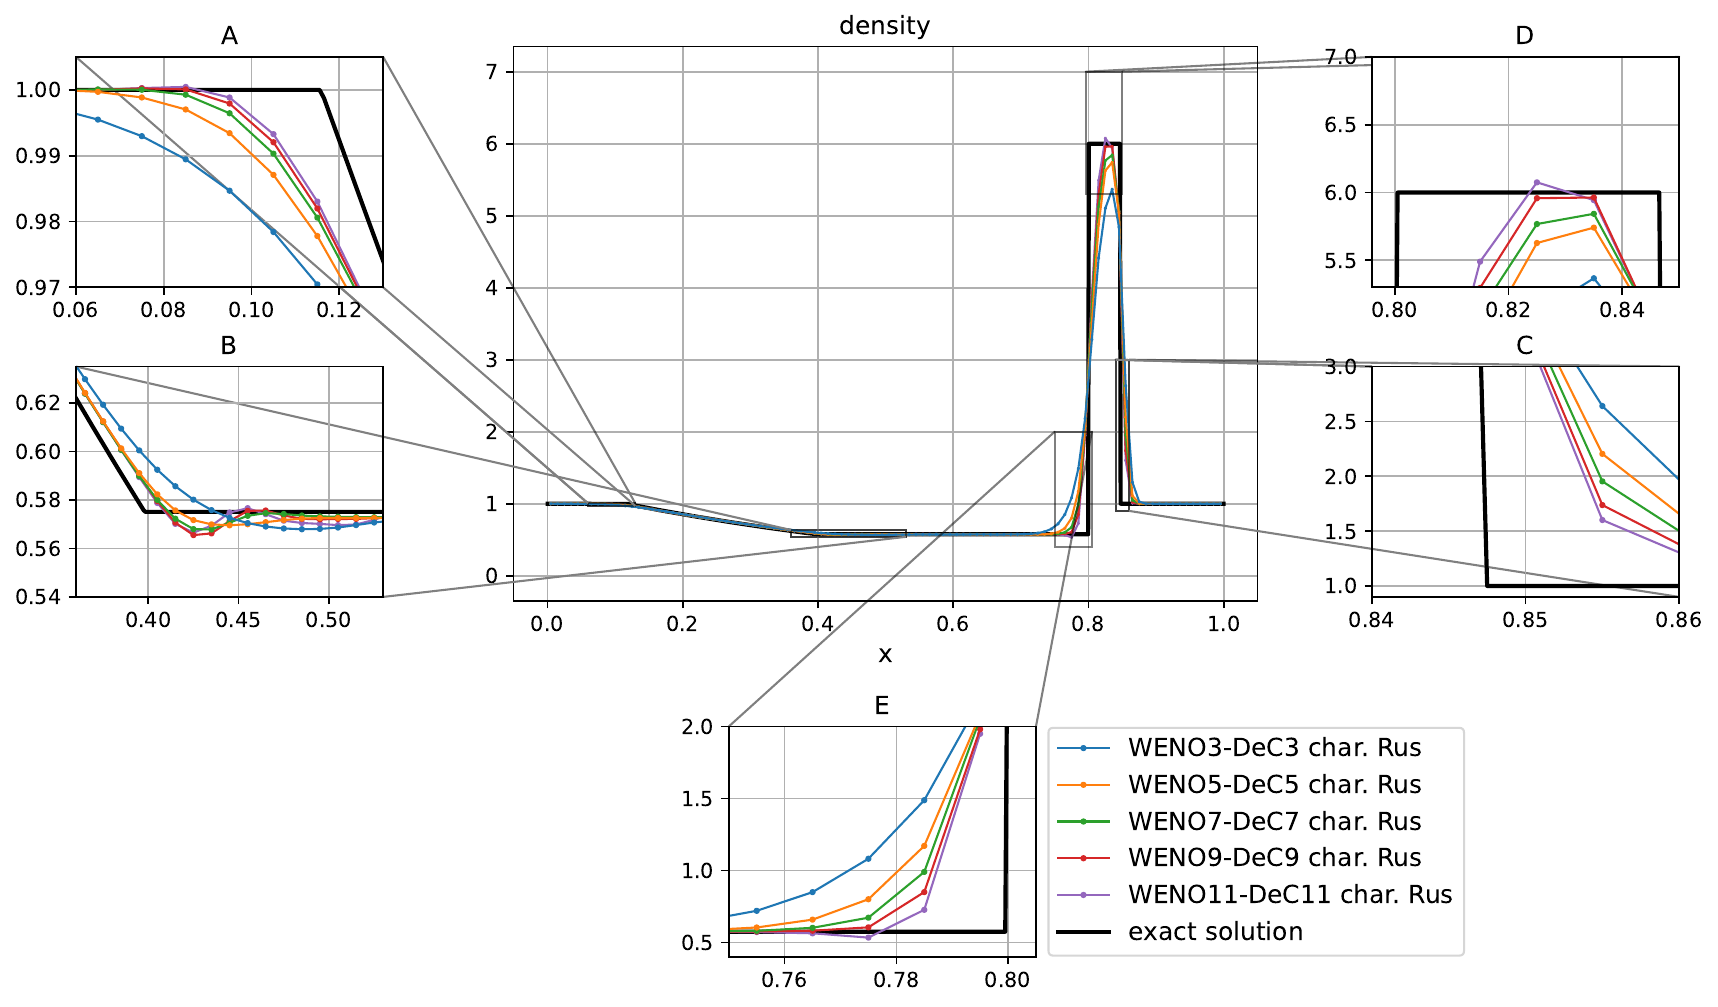}
		\caption{Reconstruction of characteristic variables and Rusanov}
	\end{subfigure}
	\\
	\begin{subfigure}[b]{0.6\textwidth}
		\centering
		\includegraphics[width=\textwidth]{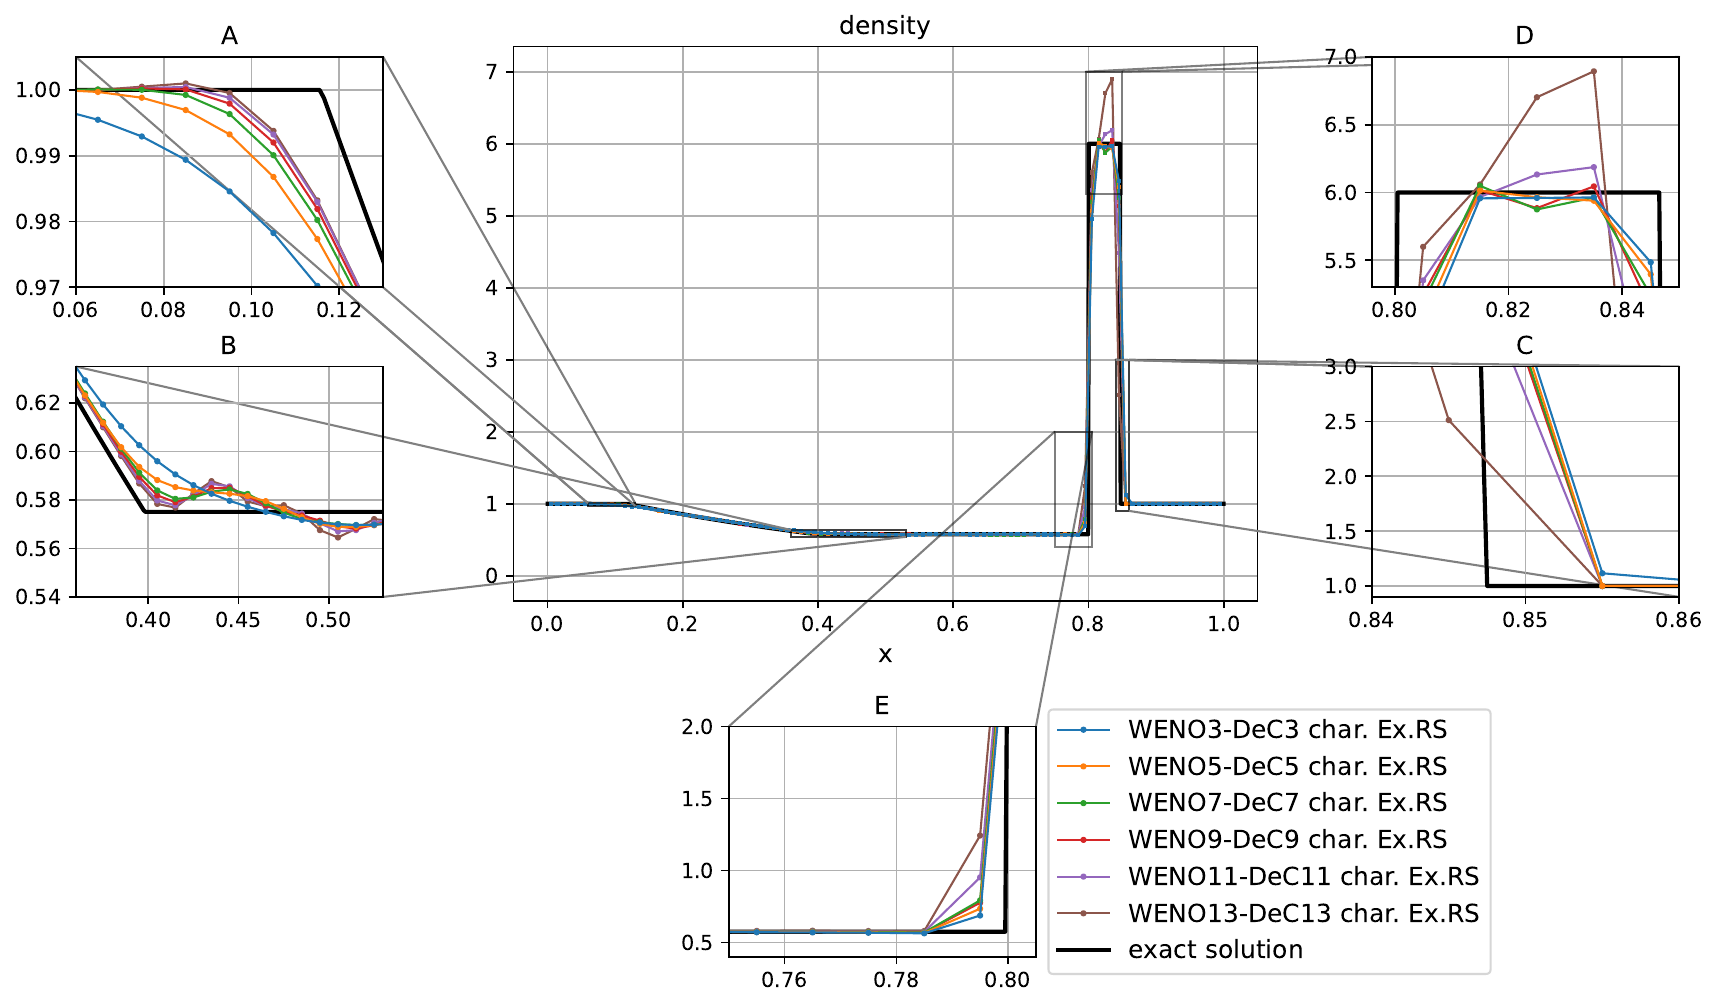}
		\caption{Reconstruction of characteristic variables and exact Riemann solver}
	\end{subfigure}
	\caption{Euler equations, Riemann problem 5: Results for the density obtained through WENO--DeC with $C_{CFL}:=0.1$}
	\label{fig:Euler_1d_RP5_zoom_density}
\end{figure}

\section{Modified shock--turbulence interaction}\label{sec:Euler_1d_titarev_toro}
In Figure~\ref{fig:Euler_1d_titarev_toro_zoom_density}, we report the results obtained for the density for all settings on the modified shock--turbulence interaction problem with $C_{CFL}:=0.95$.

\begin{figure}[htbp]
	\centering
	\begin{subfigure}[b]{0.45\textwidth}
		\centering
		\includegraphics[width=\textwidth]{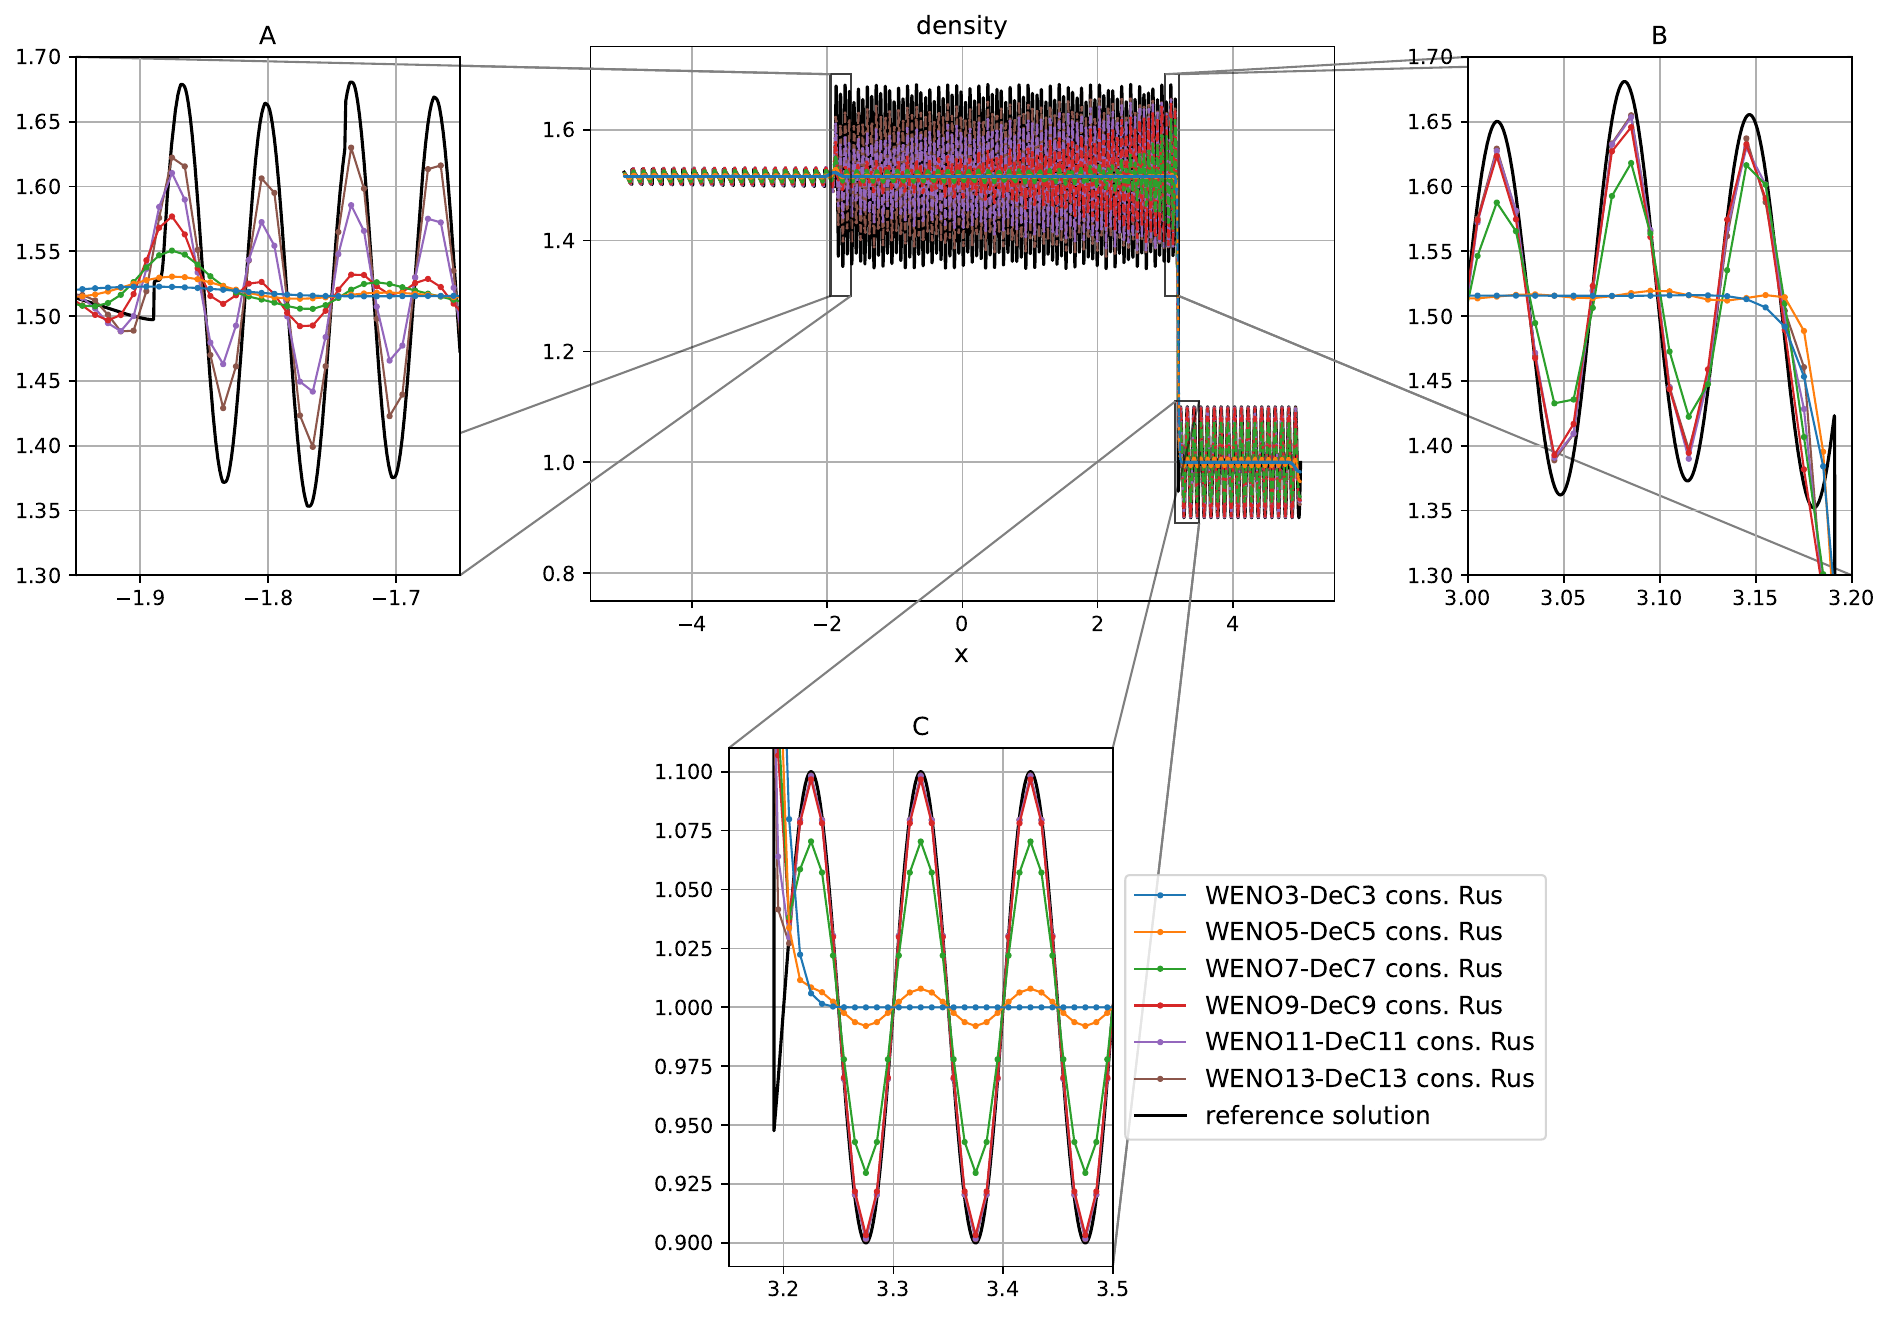}
		\caption{Reconstruction of conserved variables and Rusanov}
	\end{subfigure}
	\hfill
	\begin{subfigure}[b]{0.45\textwidth}
		\centering
		\includegraphics[width=\textwidth]{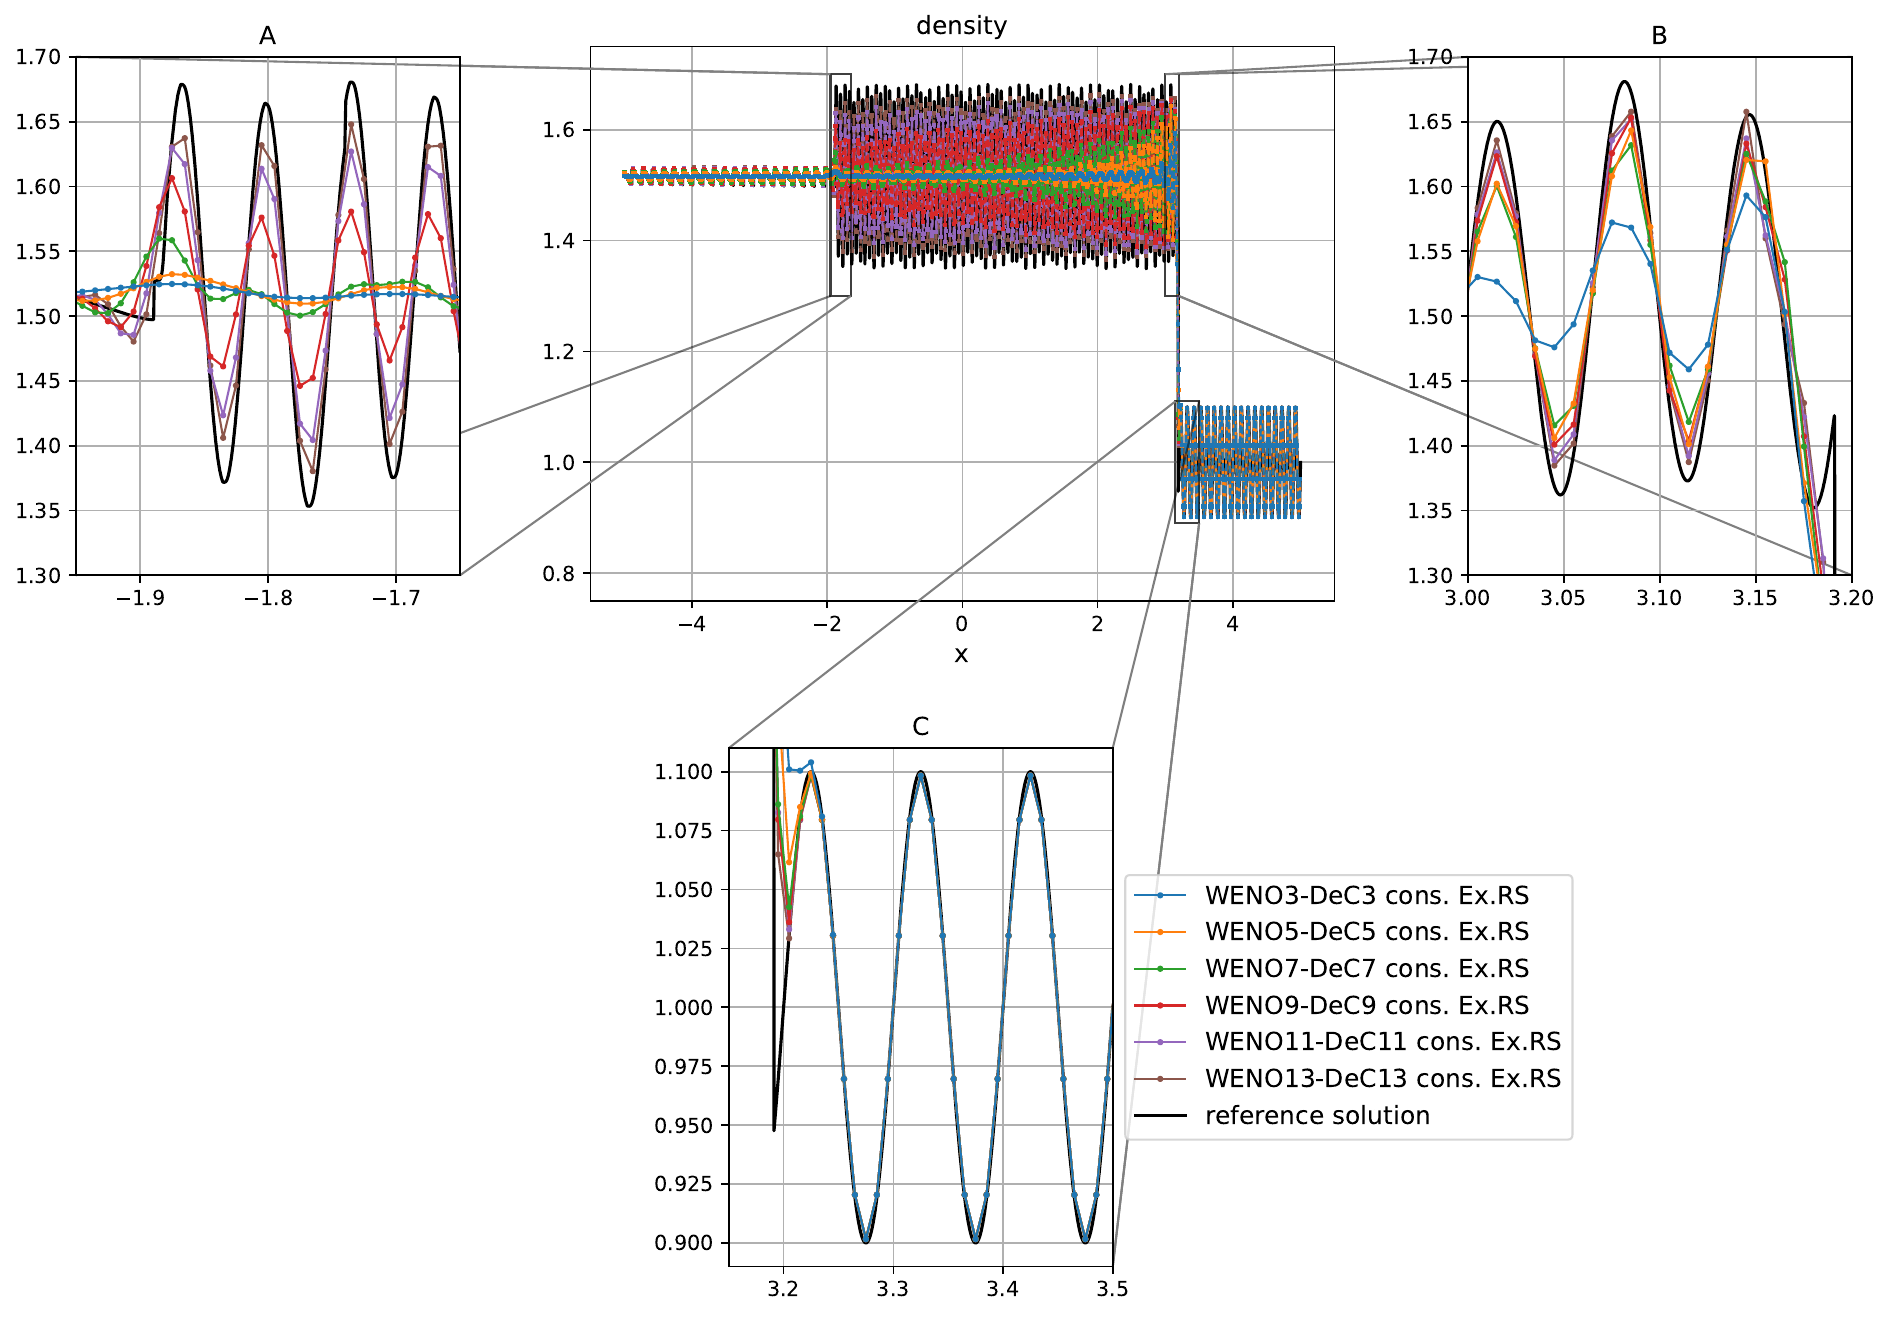}
		\caption{Reconstruction of conserved variables and exact Riemann solver}
	\end{subfigure}
	\\
	\begin{subfigure}[b]{0.45\textwidth}
		\centering
		\includegraphics[width=\textwidth]{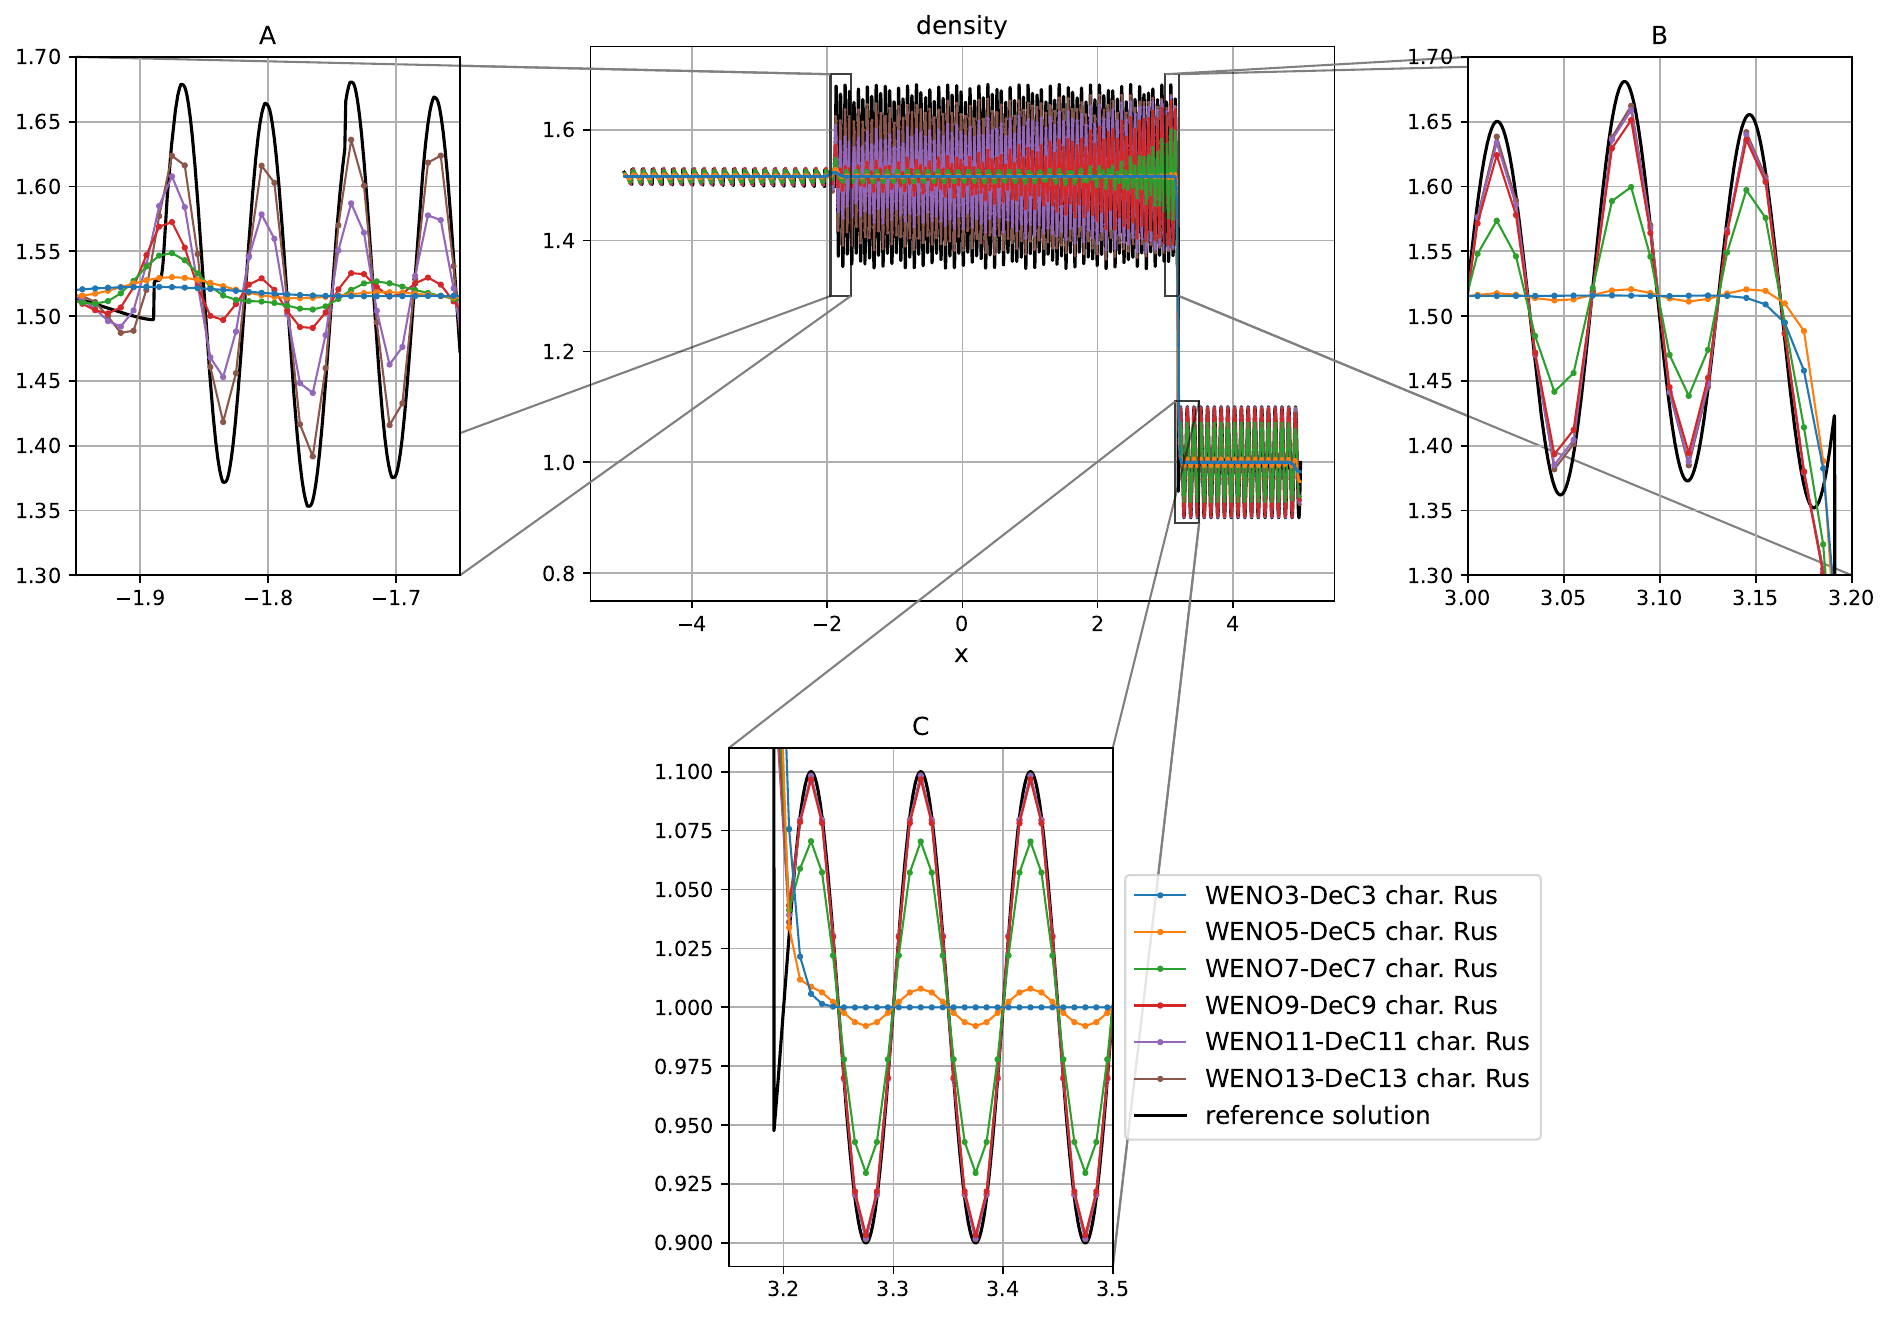}
		\caption{Reconstruction of characteristic variables and Rusanov}
	\end{subfigure}
	\hfill
	\begin{subfigure}[b]{0.45\textwidth}
		\centering
		\includegraphics[width=\textwidth]{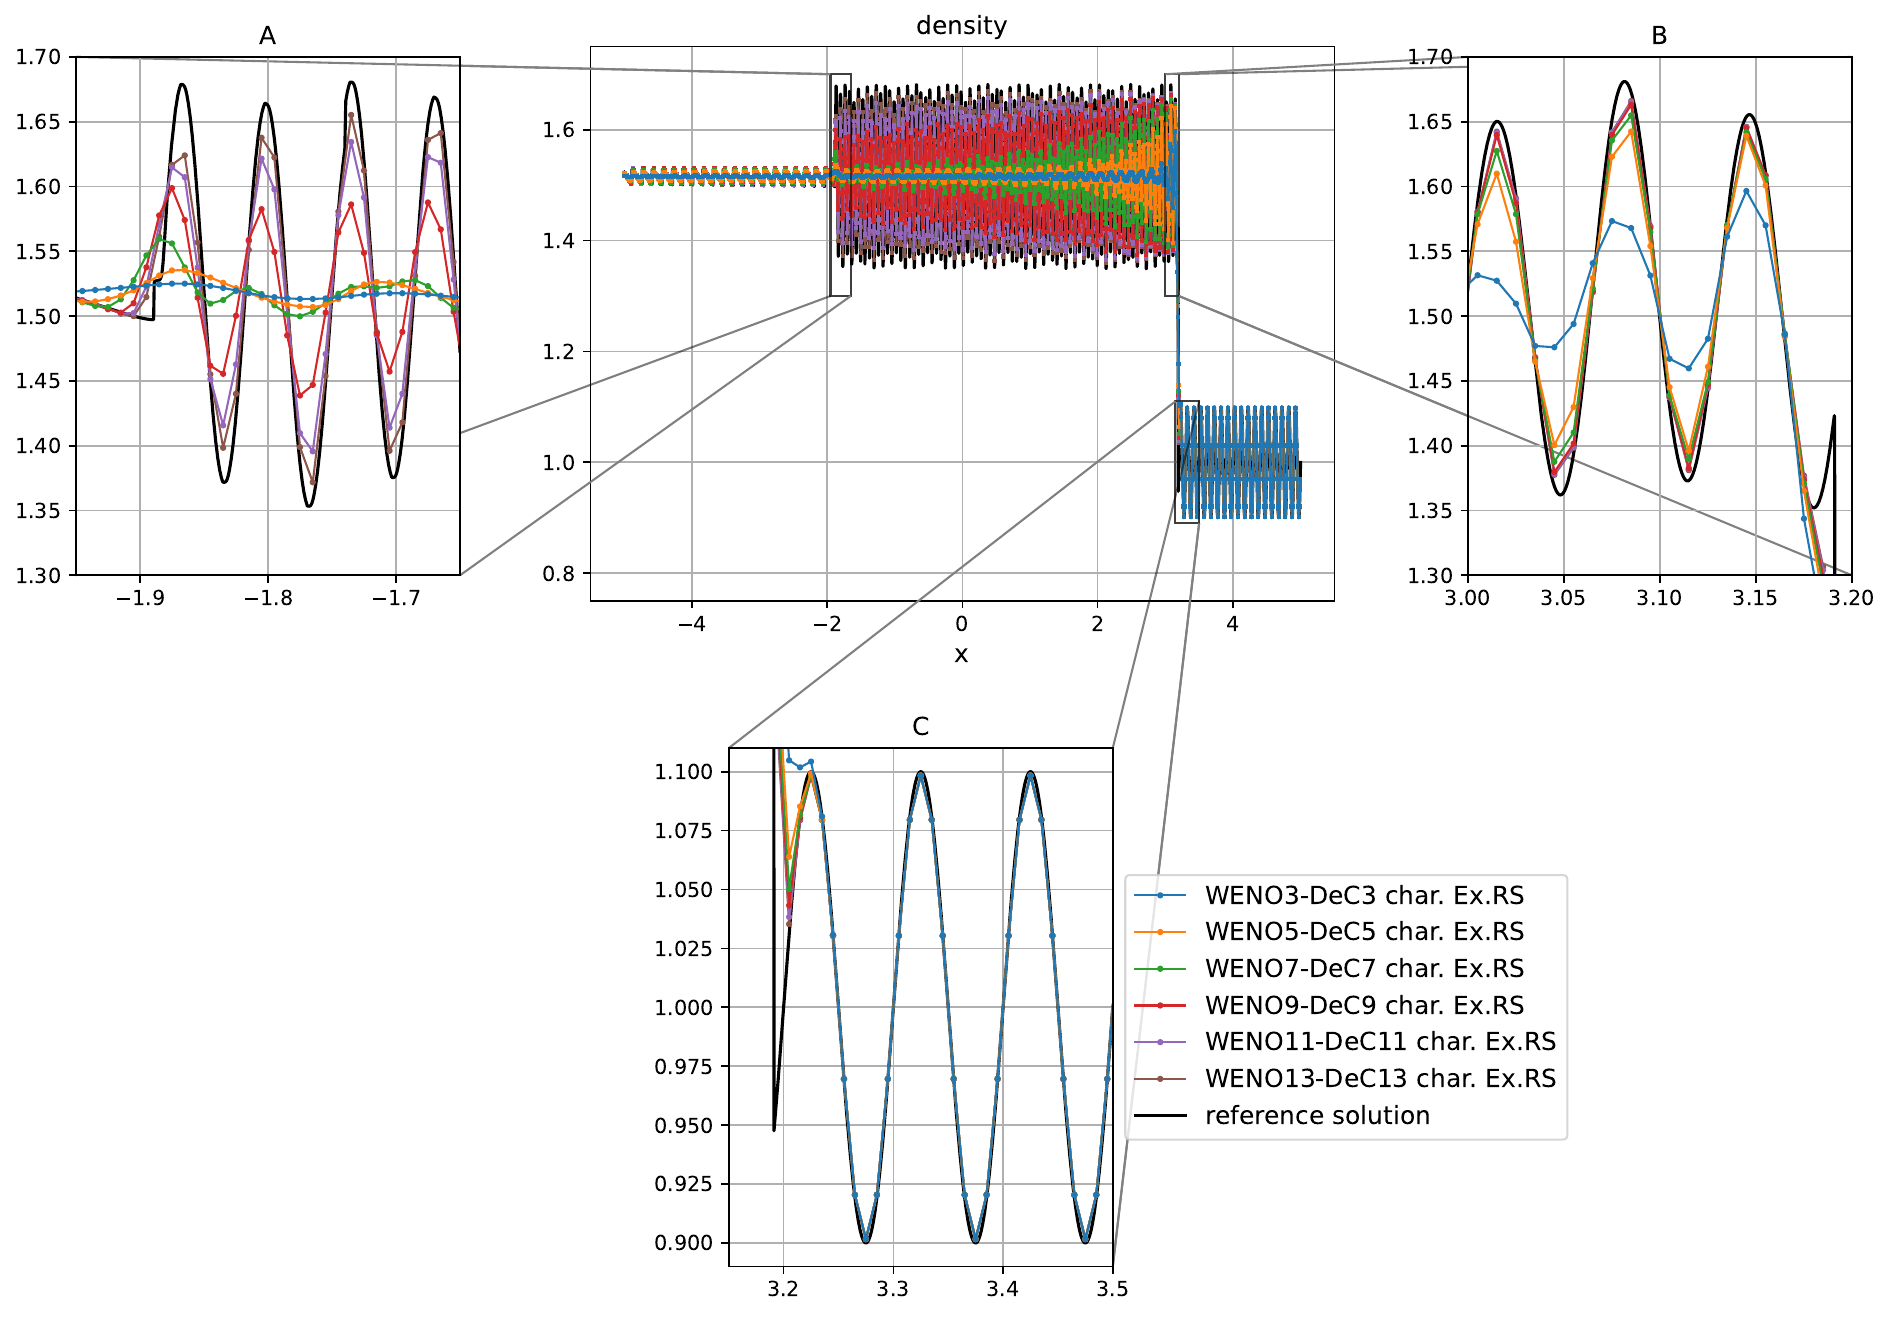}
		\caption{Reconstruction of characteristic variables and exact Riemann solver}
	\end{subfigure}
	\caption{Euler equations, Modified shock--turbulence interaction: Results for the density obtained through WENO--DeC with $C_{CFL}:=0.95$}
	\label{fig:Euler_1d_titarev_toro_zoom_density}
\end{figure}

\printbibliography

\end{document}
